# Supplementary material for: A method to evaluate the reliability of social media data for social network analysis
Source: arXiv:2010.08717 source file (2020-10-17)
Supplement: Supplementary file 1 [file appendix.tex]

\newpage
\section*{Appendix 1: Extra Stuff}

\lm{Suggest leaving the Appendix out entirely. It's basically all about a different study, which doesn't add much to the points already made in the main paper (although is an interesting dataset in its own right). Let's save the dataset for a different paper!} \dcw{+1}

More detail

\begin{table}[ht]
    \centering%\scriptsize
    \resizebox{\textwidth}{!}{%
    \begin{tabular}{lllclr}
        \toprule
        Collection   & Filter terms               & Tool   & Duration (hrs) & Period     & Posts \\
        \midrule
    	Q\&A Part 1  & qanda\textsuperscript{$*$} & RAPID  & 4              & 8 Nov 2018 & 15930 \\
    	             &                            & Twarc  &                &            & 27389 \\ \cmidrule{2-6}
    	Q\&A Part 2  & qanda\textsuperscript{$*$} & RAPID  & 15             & 9 Nov 2018 & 11719 \\
    	             &                            & Twarc  &                &            & 15490 \\ \midrule
        AFL1         & afl                        & RAPID  & 72             & March 2019 & 21799 \\
    	             &                            & Twarc  &                &            & 44470 \\ \cmidrule{2-6}
        AFL2         & afl                        & RAPID  & 144            & April 2019 & 30103 \\
    	             &                            & RAPID  &                &            & 30115 \\
        Election Day & \hl{nswelection, nswvotes} & RAPID  & 24             & March 2019 & 39556 \\
    	             & \hl{nswpol, nswvotes2019}  & Twarc  &                &            & 39297 \\
    	             &                            & Tweepy &                &            & 36172 \\
        \bottomrule
    \end{tabular}
    } % end resizebox/textwidth
    \caption{Broad details of Twitter collections conducted for this study. \textsuperscript{$*$}Other terms were used which are not included here for privacy reasons.} % turnbull, turnbullmalcolm
    \label{tab:twitter_collections_expanded}
\end{table}

% \color{red}Should tables \ref{tab:dataset_stats1} and \ref{tab:dataset_stats2} go in the appendix?\color{black}

\begin{sidewaystable}
%\begin{table}[ht]
\centering\tiny
\begin{tabular}{lrrrrrr}
    \toprule
    & AFL1  & AFL1  & AFL1-en & AFL1-en & AFL2a & AFL2b  \\
    & RAPID & Twarc & RAPID   & Twarc   &       &        \\
    \midrule
    tweet\_count & 21799 & 44470 & 21534 & 27051 & 30103 & 30115 \\
    retweet\_count & 7047 & 11482 & 6965 & 8262 & 9215 & 9215 \\
    quote\_count & 1670 & 2658 & 1653 & 2363 & 2340 & 2341 \\
    reply\_count & 6060 & 6516 & 6018 & 6313 & 9229 & 9229 \\
    tweets\_with\_hashtags & 7119 & 10243 & 7026 & 8290 & 8623 & 8627 \\
    tweets\_with\_urls & 7504 & 26512 & 7388 & 11414 & 11467 & 11474 \\
    author\_count & 11573 & 16821 & 11377 & 12836 & 14231 & 14232 \\
    %most\_prolific\_author & 1060063613459685376 & 1048457428063272961 & 1060063613459685376 & 1048457428063272961 & 18892137 & 18892137 \\
    most\_prolific\_author\_tweet\_count & 362 & 1123 & 362 & 1123 & 612 & 612 \\
    %most\_retweeted\_tweet & 1109062149890936833 & 1108983100028145664 & 1109062149890936833 & 1109062149890936833 & 1113316916775387136 & 1113316916775387136 \\
    most\_retweeted\_tweet\_count & 529 & 1293 & 529 & 529 & 269 & 269 \\
    %most\_replied\_to\_tweet & 1109239950145437696 & 1109239950145437696 & 1109239950145437696 & 1109239950145437696 & 1113291142634725377 & 1113291142634725377 \\
    most\_replied\_to\_tweet\_count & 144 & 144 & 144 & 144 & 206 & 206 \\
    tweets\_with\_mentions & 15579 & 20795 & 15435 & 17336 & 22083 & 22083 \\
    %most\_mentioned\_author & 16319888 & 16319888 & 16319888 & 16319888 & 16319888 & 16319888 \\
    most\_mentioned\_author\_count & 7259 & 7261 & 7253 & 7255 & 10468 & 10468 \\
    hashtags\_uses & 16289 & 23426 & 16004 & 18431 & 20136 & 20140 \\
    unique\_hashtags & 2360 & 3498 & 2262 & 2770 & 3337 & 3337 \\
    most\_used\_hashtag & afl & afl & afl & afl & afl & afl \\
    most\_used\_hashtag\_count & 4600 & 4603 & 4561 & 4563 & 5096 & 5096 \\
    urls\_uses & 3659 & 23051 & 3589 & 7690 & 5702 & 5709 \\
    unique\_urls & 2128 & 10403 & 2073 & 4188 & 3580 & 3587 \\
    %most\_used\_url & \url{http://watchrugby.net/AFL/} & \url{http://watchrugby.net/AFL/} & \url{http://watchrugby.net/AFL/} & \url{http://watchrugby.net/AFL/} & \url{http://watchrugby.net/AFL/} & \url{http://watchrugby.net/AFL/}F \\
    most\_used\_url\_count & 251 & 494 & 251 & 494 & 341 & 341 \\
    \bottomrule
\end{tabular}
\caption{``AFL''-related dataset statistics.}
\label{tab:dataset_stats1}

\bigskip\bigskip % space between tables
\begin{tabular}{lrrrrrrr}
    \toprule
    & Election Day & Election Day & Election Day & Q\&A1 & Q\&A1 & Q\&A2 & Q\&A2 \\
    & RAPID        & Twarc        & Tweepy       & RAPID & Twarc & RAPID & Twarc \\
    \midrule
    tweet\_count & 39556 & 39297 & 36172 & 15930 & 27389 & 11719 & 15490 \\
    retweet\_count & 26612 & 26412 & 24276 & 8744 & 27389 & 8051 & 15490 \\
    quote\_count & 3610 & 3590 & 3363 & 325 & 1203 & 498 & 1232 \\
    reply\_count & 1381 & 1374 & 1252 & 1446 & 2067 & 1715 & 1731 \\
    tweets\_with\_hashtags & 21686 & 21582 & 19977 & 10043 & 15591 & 3912 & 3961 \\
    tweets\_with\_urls & 7860 & 7829 & 7194 & 2470 & 4029 & 3106 & 4074 \\
    author\_count & 10893 & 10860 & 10242 & 4970 & 7057 & 4708 & 5799 \\
    %most\_prolific\_author & 10482452 & 10482452 & 10482452 & 47239788 & 47239788 & 922361848703328257 & 17353325 \\
    most\_prolific\_author\_tweet\_count & 211 & 212 & 212 & 103 & 146 & 57 & 68 \\
    %most\_retweeted\_tweet & 1109036231931781120 & 1109036231931781120 & 1109036231931781120 & 1060464094434680834 & 1060464094434680834 & 1060624846915198976 & 1060624846915198976 \\
    most\_retweeted\_tweet\_count & 367 & 368 & 278 & 260 & 288 & 385 & 385 \\
    %most\_replied\_to\_tweet & 1109193310483079168 & 1109193310483079168 & 1109193310483079168 & 1060456782181490689 & 1060456782181490689 & 1060671176328900610 & 1060671176328900610 \\
    most\_replied\_to\_tweet\_count & 26 & 25 & 24 & 55 & 121 & 58 & 58 \\
    tweets\_with\_mentions & 30848 & 30626 & 28154 & 11314 & 18253 & 10472 & 13514 \\
    %most\_mentioned\_author & 704882735815401472 & 704882735815401472 & 704882735815401472 & 16734909 & 16734909 & 16734909 & 16734909 \\
    most\_mentioned\_author\_count & 2443 & 2442 & 2187 & 2883 & 3853 & 2753 & 2752 \\
    hashtags\_uses & 51470 & 51288 & 47106 & 15700 & 23557 & 7672 & 7862 \\
    unique\_hashtags & 2458 & 2450 & 2306 & 1015 & 1438 & 960 & 1082 \\
    most\_used\_hashtag & nswvotes & nswvotes & nswvotes & qanda & qanda & qanda & qanda \\
    most\_used\_hashtag\_count & 11731 & 11739 & 10901 & 10065 & 15644 & 2545 & 2549 \\
    urls\_uses & 3761 & 3766 & 3478 & 913 & 1650 & 1602 & 2411 \\
    unique\_urls & 1374 & 1374 & 1258 & 399 & 560 & 658 & 790 \\
    %most\_used\_url & \url{https://www.fiverr.com/s2/da1254eff6} & \url{https://www.fiverr.com/s2/da1254eff6} & \url{https://www.fiverr.com/s2/da1254eff6} & \url{http://wp.me/p2WW3S-Gg} & \url{http://wp.me/p2WW3S-Gg} & \url{https://twitter.com/qanda/status/1060469840664702977?s=21} & \url{https://twitter.com/skynewsaust/status/1060648691759951872} \\
    most\_used\_url\_count & 100 & 100 & 100 & 49 & 128 & 71 & 81 \\
    \bottomrule
\end{tabular}
\caption{``Election Day'' and ``Q\&A''-related dataset statistics.}
\label{tab:dataset_stats2}
%\end{table}
\end{sidewaystable}

\begin{table}[ht]
    \centering\scriptsize
    \begin{tabular}{llrrc}
        \toprule
        Collection   & Interaction & Nodes & Edges &  ARI  \\
        \midrule
        AFL1-en      & RETWEET     &  5653 &  5936 & 0.818 \\
                     & MENTION     & 11692 & 21875 & 0.675 \\
                     & REPLY       &  4747 &  4627 & 0.853 \\
        Election Day & RETWEET     &  8618 & 22868 & 0.527 \\
                     & MENTION     & 10115 & 36111 & 0.632 \\
                     & REPLY       &  1232 &  1168 & 0.784 \\
        % Election Day   & RETWEET   &  8193 & 22286 & 0.396 \\
        % (Twarc/Tweepy) & MENTION   &  9600 & 35235 & 0.602 \\
        %                & REPLY     &  1147 &  1094 & 0.597 \\
        Q\&A Part 1  & RETWEET     &  3232 &  7840 & 0.320 \\
                     & MENTION     &  4529 & 12969 & 0.350 \\
                     & REPLY       &  1183 &  1490 & 0.738 \\
        Q\&A Part 2  & RETWEET     &  3555 &  7924 & 0.437 \\
                     & MENTION     &  5152 & 14577 & 0.468 \\
                     & REPLY       &  1487 &  1499 & 0.756 \\
        \bottomrule
    \end{tabular}
    \caption{Comparison of the communities found in the networks built from the RAPID and Twarc datasets for several collections. The node count is the number of nodes in common between the networks, the edge count is drawn from the RAPID dataset in each case, to give an indication of density, and the ``ARI'' value is the Adjusted Rand index.}
    \label{tab:community_comparison_expanded}
\end{table}

\textbf{Q\&A centrality scatter plots}

\textbf{AFL centrality scatter plots}

\textbf{Election Day}

\subsection*{Case Study 4: Election Day}

\textbf{WHAT IF WE USE ANOTHER TOOL THAT SHOULD BE IDENTICAL TO TWARC: TWEEPY}

\emph{Effects on centrality measures}

More pertinent to this study is the question of how the variations in collections affect the social networks that SNA researchers build from their data. Is it possible that even if collections may differ, are social networks built from their data robust? Are some networks, based on one kind of interaction or edge-connection criteria, more robust than others? One primary approach to examining a social network is to consider centrality measures of the nodes of the networks constructed. If the networks are robust then, although centrality measures may change due to topological differences, their ranking ought to remain relatively similar.

\textbf{Centrality comparisons of mention and reply networks}

Using ``AFL1-en'' and ``Election Day'' datasets, we constructed weighted directed networks from the reply and mention interactions. Nodes in these networks are user accounts, connected by a weighted directed edge from the replier or mentioner to the replied to or mentioned account, and weighted by the number of such interactions in the dataset. We then calculated degree centrality, betweenness, closeness and eigenvector centrality values for each of the nodes in each network, and these were then ranked in order. If the networks are robust, then the centrality rankings for the ``AFL1-en'' and the ``Election Day'' RAPID and Twarc collections should be very similar, respectively, though more variation is likely further down the lists.

Figures \ref{fig:afl1_centrality_ranking_comparisons} and \ref{fig:elec_centrality_ranking_comparisons} show the ranking comparisons for the top at most 1000 common nodes of the ``AFL1-en'' and ``Election Day'' collections (all above 800 nodes in common). Each node's $(x,y)$ coordinate is determined by its centrality ranking in each of the RAPID- and Twarc-derived graphs, and the greyscale value corresponds to their position on the RAPID (horizontal) list (darker ranks are higher). The predominant linear nature of the plots indicates that the majority of nodes held the same rank across both graphs, while the fork patterns is a symptom of nodes with differing ranks. The more items are out of their linear ranking, say because their rankings improve in the second list, the more they displace other items, which are necessarily placed lower in the second list, therefore for each dot above the linear in the chart, there is a corresponding one somewhere below it. Furthermore, the more robust a network measure is, the farther down the list the divergence occurs.

\begin{figure}[ht!]
    \centering
    \includegraphics[scale=0.35]{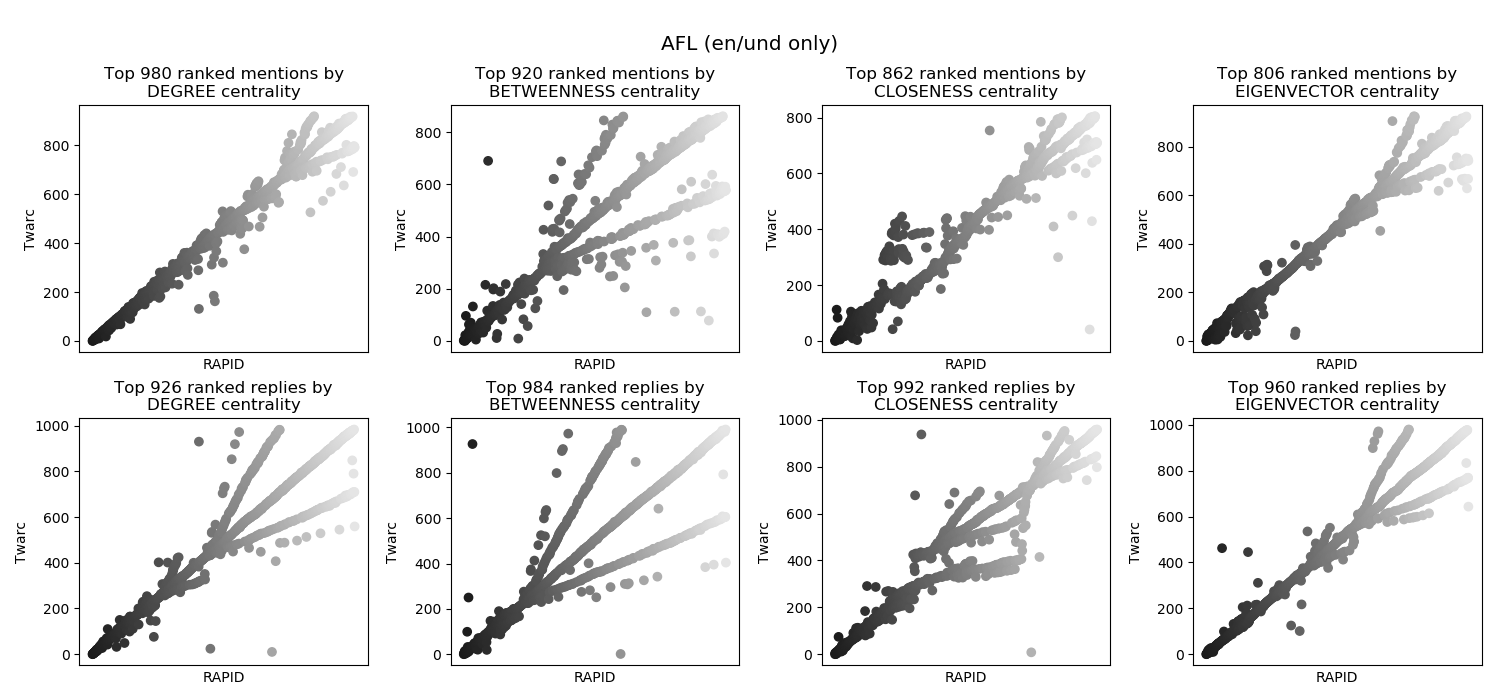}
    \caption{Centrality ranking comparisons from the RAPID and Twarc datasets of the ``AFL1-en'' collection.}
    \label{fig:afl1_centrality_ranking_comparisons}
\end{figure}

\begin{figure}[ht!]
    \centering
    \includegraphics[scale=0.35]{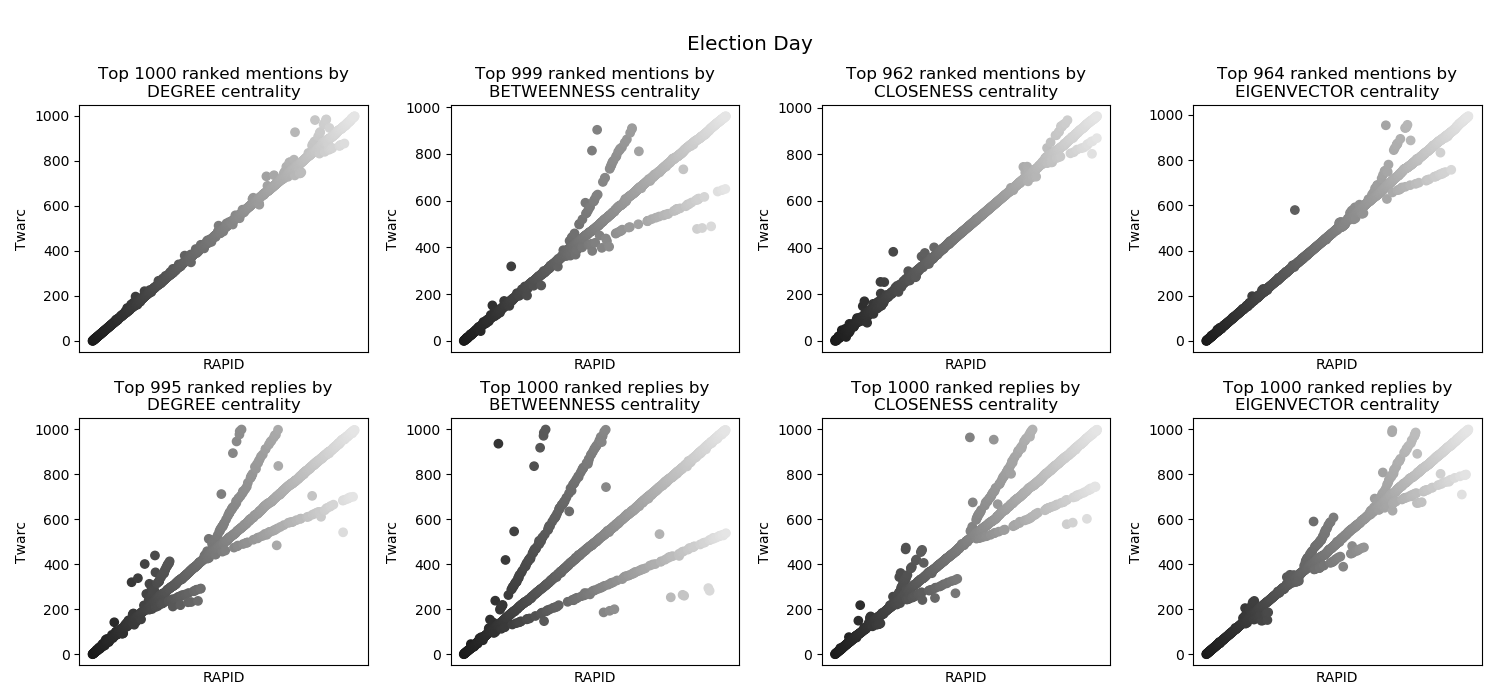}
    \caption{Centrality ranking comparisons from the RAPID and Twarc datasets of the ``Election Day'' collection.}
    \label{fig:elec_centrality_ranking_comparisons}
\end{figure}

The mentions networks are relatively robust for both collections, apart from the betweenness measure, which diverges after about a third, compared with the reply networks, which diverge sooner. Because betweenness centrality is sensitive to topology, it is understandably more sensitive to variations in collection, as compared with the other measures. Reply networks are more reliant on the nature of conversations, as they require a post to which to reply (in contrast, original posts can mention other users without any such instigation). The forking observed in the reply networks seems more consistent, as if nodes which vary in rank almost literally swap, rather than displace one another.

\textbf{Varying the comparison plot algorithm}

Attempts were made to counter the forking effect by devising a plotting algorithm that would reward nodes which retained their neighbourhood, or context, even if nodes above or below changed rank. This method was inspired by part of the Kendall Tau similarity calculation and assigns a value for each ranked item in the second list based on the item's location in the first. The value is equal to the number of items that have a lower ranking than the current item than the first list that appear below the current item in the second list. I.e., if an item lower ranked than the current one appears above it in the second list, the item's score goes down by one - in contrast, the ranking of all items below the moved item in the second list have a different ranking. The result is that the Twarc scores will always be the same or lower than the RAPID ranking and higher ranked nodes are located to the top right, rather than the bottom left. The intent of the algorithm is to keep items on the linear path if their neighbours remain the same.

\begin{figure}[ht!]
    \centering
    \includegraphics[scale=0.35]{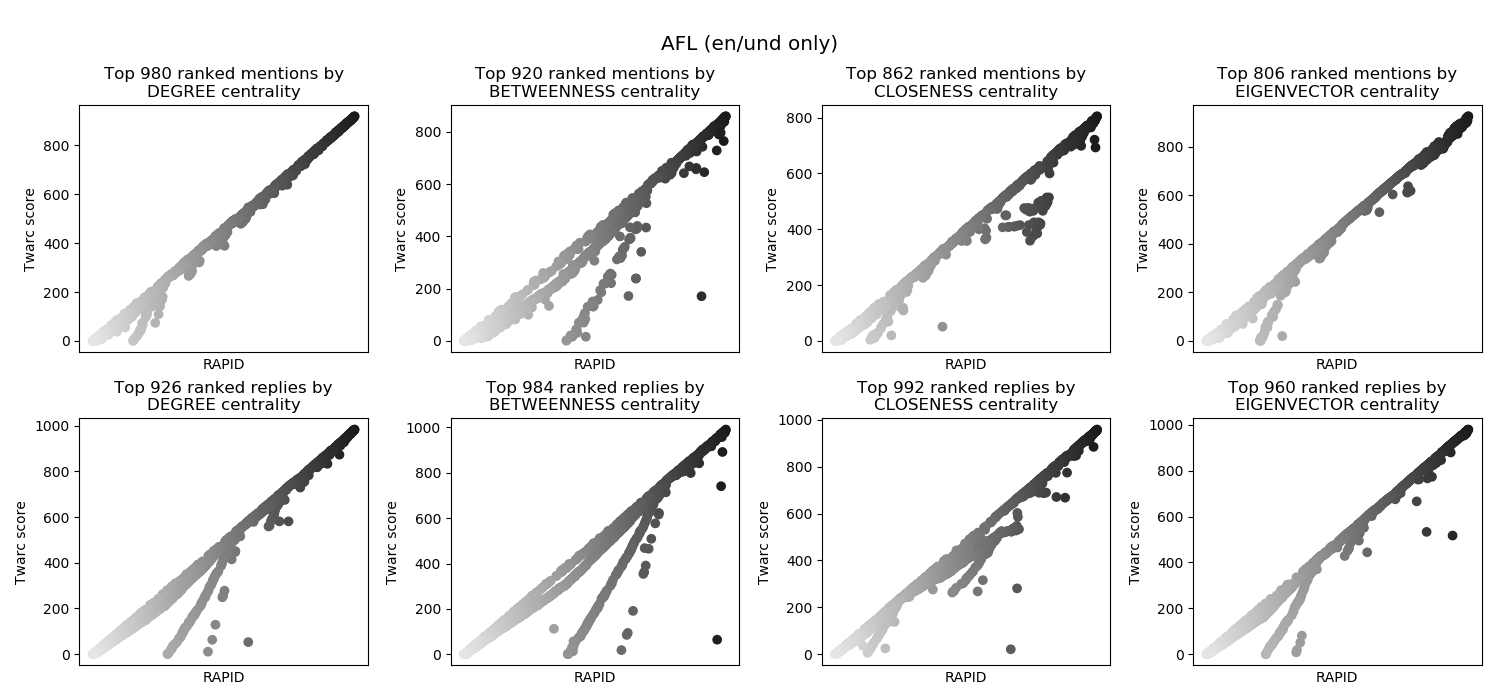}
    \caption{Centrality ranking comparisons from the RAPID and Twarc datasets of the ``AFL1-en'' collection with the ranking variation.}
    \label{fig:afl1_centrality_ranking_comparisons2}
\end{figure}

\begin{figure}[ht!]
    \centering
    \includegraphics[scale=0.35]{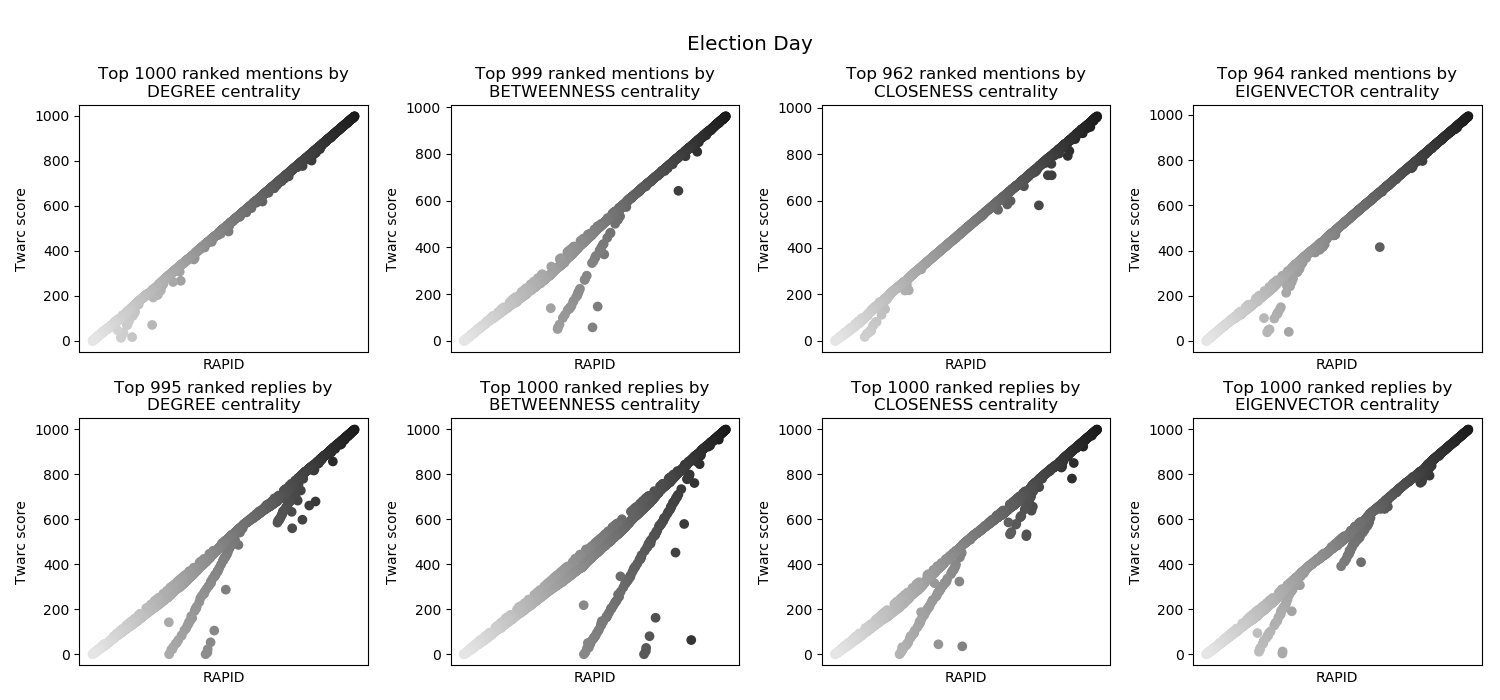}
    \caption{Centrality ranking comparisons from the RAPID and Twarc datasets of the ``Election Day'' collection with the ranking variation.}
    \label{fig:elec_centrality_ranking_comparisons2}
\end{figure}

Figures \ref{fig:afl1_centrality_ranking_comparisons2} and \ref{fig:elec_centrality_ranking_comparisons2} show the comparisons between rankings for ``ALF1-en'' and ``Election Day''. These charts highlight the fact that relatively few nodes are out of place - most of the rankings are preseved for both mention and reply networks, though there are communities of nodes appearing out of their rankings by the same degree (e.g., in the closeness centralities for the ``AFL1-en'' mention network and the degree centrality for the ``Election Day'' reply network).

\textbf{Similarity measures}

A quantitive approach to comparing the centrality rankings of the networks of the ``AFL1-en'' and ``Election Day'' collections was also considered, making use of Kendall Tau scores and Spearman's Coeffecient. Although the plotted ranking comparison above provide the sense that the networks are relatively robust, because the majority of points appear on the linear path (XXX DCW: I'm not sure how to phrase this), the quantitive analyses using Kendall Tau and Spearman's Coefficient similarity measures paint another picture. As can be seen in Figures \ref{fig:afl_centrality_ranking_comparisons_tau_rho} and \ref{fig:elec_centrality_ranking_comparisons_tau_rho}, the reply networks have higher similarity scores than the mention networks across both collections, though the Kendall Tau scores around $0.4$ indicate relatively high similarity (XXX ref?). All $p$-values for $tau$ and $rho$ scores were less than $0.001$.

% \begin{figure}[t!]
%     \centering
%     \begin{subfigure}[b]{0.49\textwidth}
%         \centering
%         \includegraphics[scale=0.16]{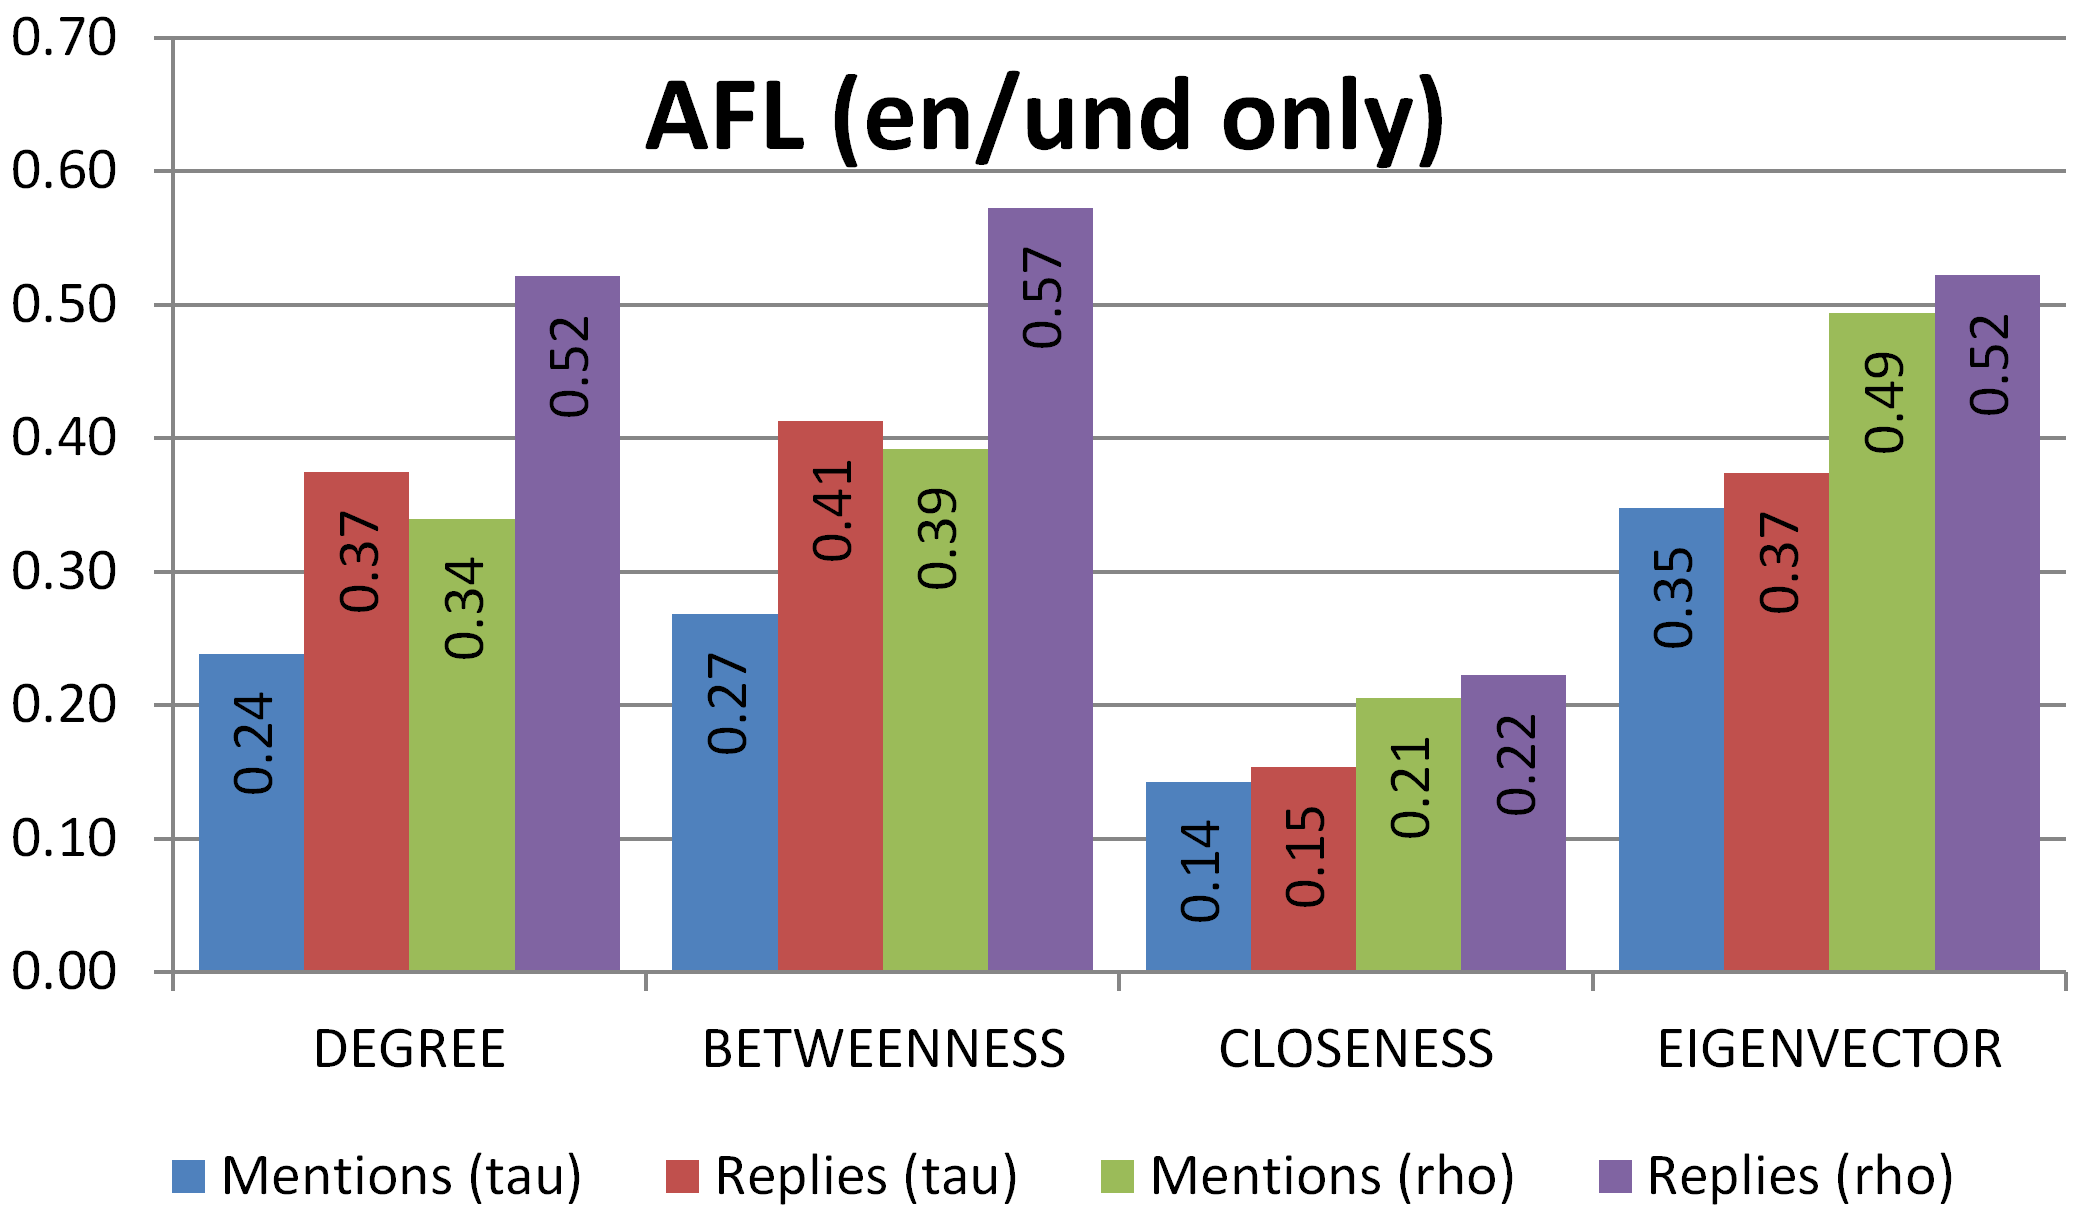}
%         \caption{``AFL1-en'' collection.}
%         \label{fig:afl_centrality_ranking_comparisons_tau_rho}
%     \end{subfigure}
%     \hfill
%     \begin{subfigure}[b]{0.49\textwidth}
%         \centering
%         \includegraphics[scale=0.16]{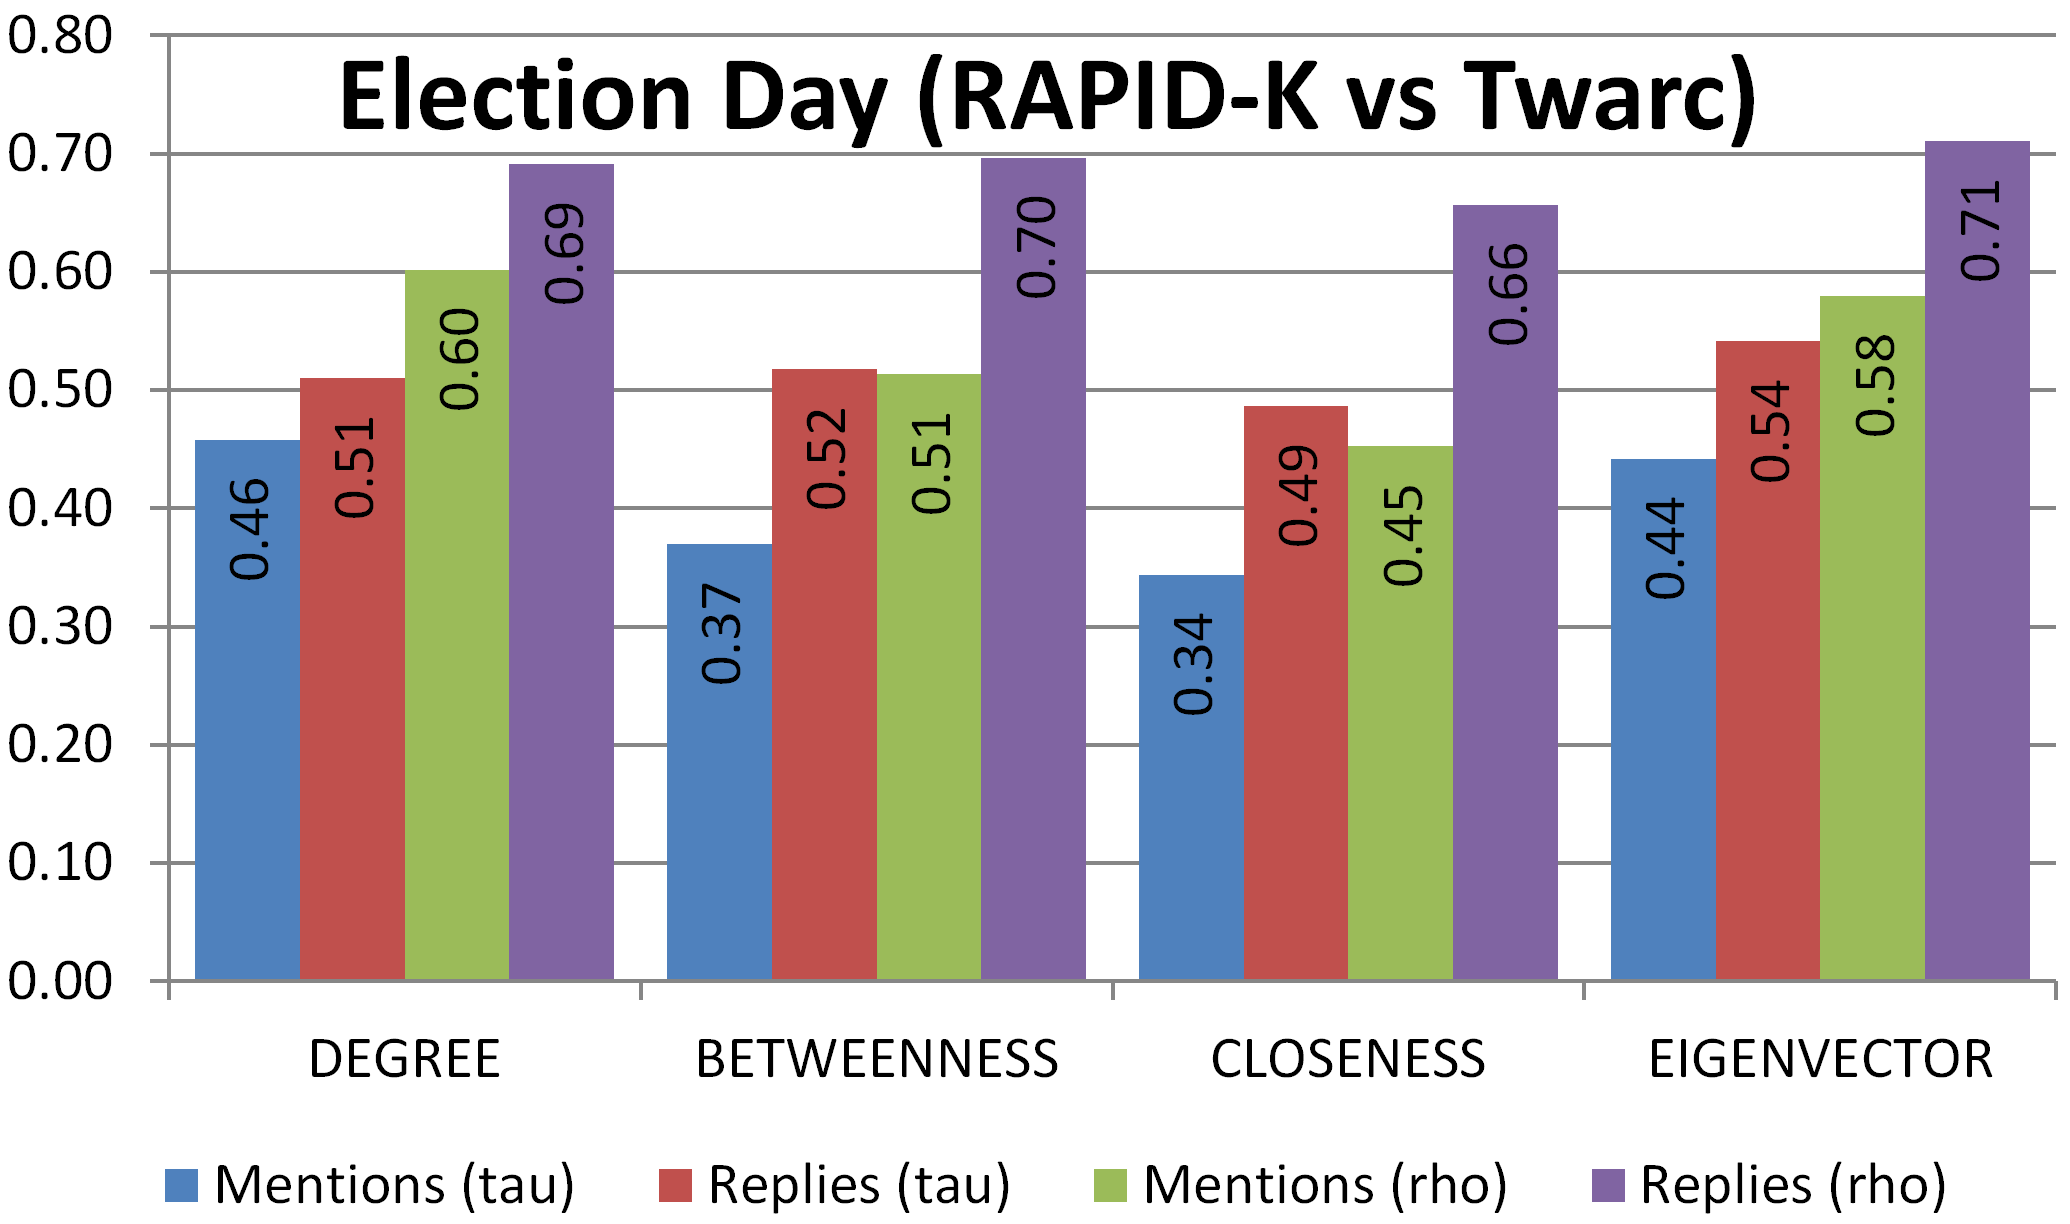}
%         \caption{``Election Day'' collection.}
%         \label{fig:elec_centrality_ranking_comparisons_tau_rho}
%     \end{subfigure}
%     \caption{Centrality ranking comparisons from the RAPID and Twarc datasets of the ``AFL1-en'' and ``Election Day'' collections using Kendall Tau scores and Spearman's Coefficients.}
% \end{figure}

DCW: I REMEMBERED ONE OF THE REASONS WHY WE STARTED ON THE DATASET RELIABILITY ANGLE WAS THAT OUR Q\&A COLLECTIONS WERE WILDLY DIFFERENT. NEED TO MAKE SURE WE MENTION THAT TOO. WILL LOOK AT THAT TOMORROW OR THE NEXT DAY.

\textbf{Longitudinal similarity}

To consider the temporal variations in collection affects similarity between collections, the Election Day dataset was broken down into 24 hour-long buckets, and the retweet, mention and reply networks derived from these were also compared for similarity of network measures. For each hour, the rankings of the top at most 1000 common nodes were compared. For the retweet network, only degree centrality was considered (XXX DOES IT NEED TO BE SPELLED OUT WHY?), while betweenness and closeness were also considered for the other networks. Eigenvector centrality was applied but found not to converge for these networks, and so is unavailable.

\begin{figure}[t!]
    \centering
    \begin{subfigure}[b]{0.3\textwidth}
        \centering
        \includegraphics[scale=0.11]{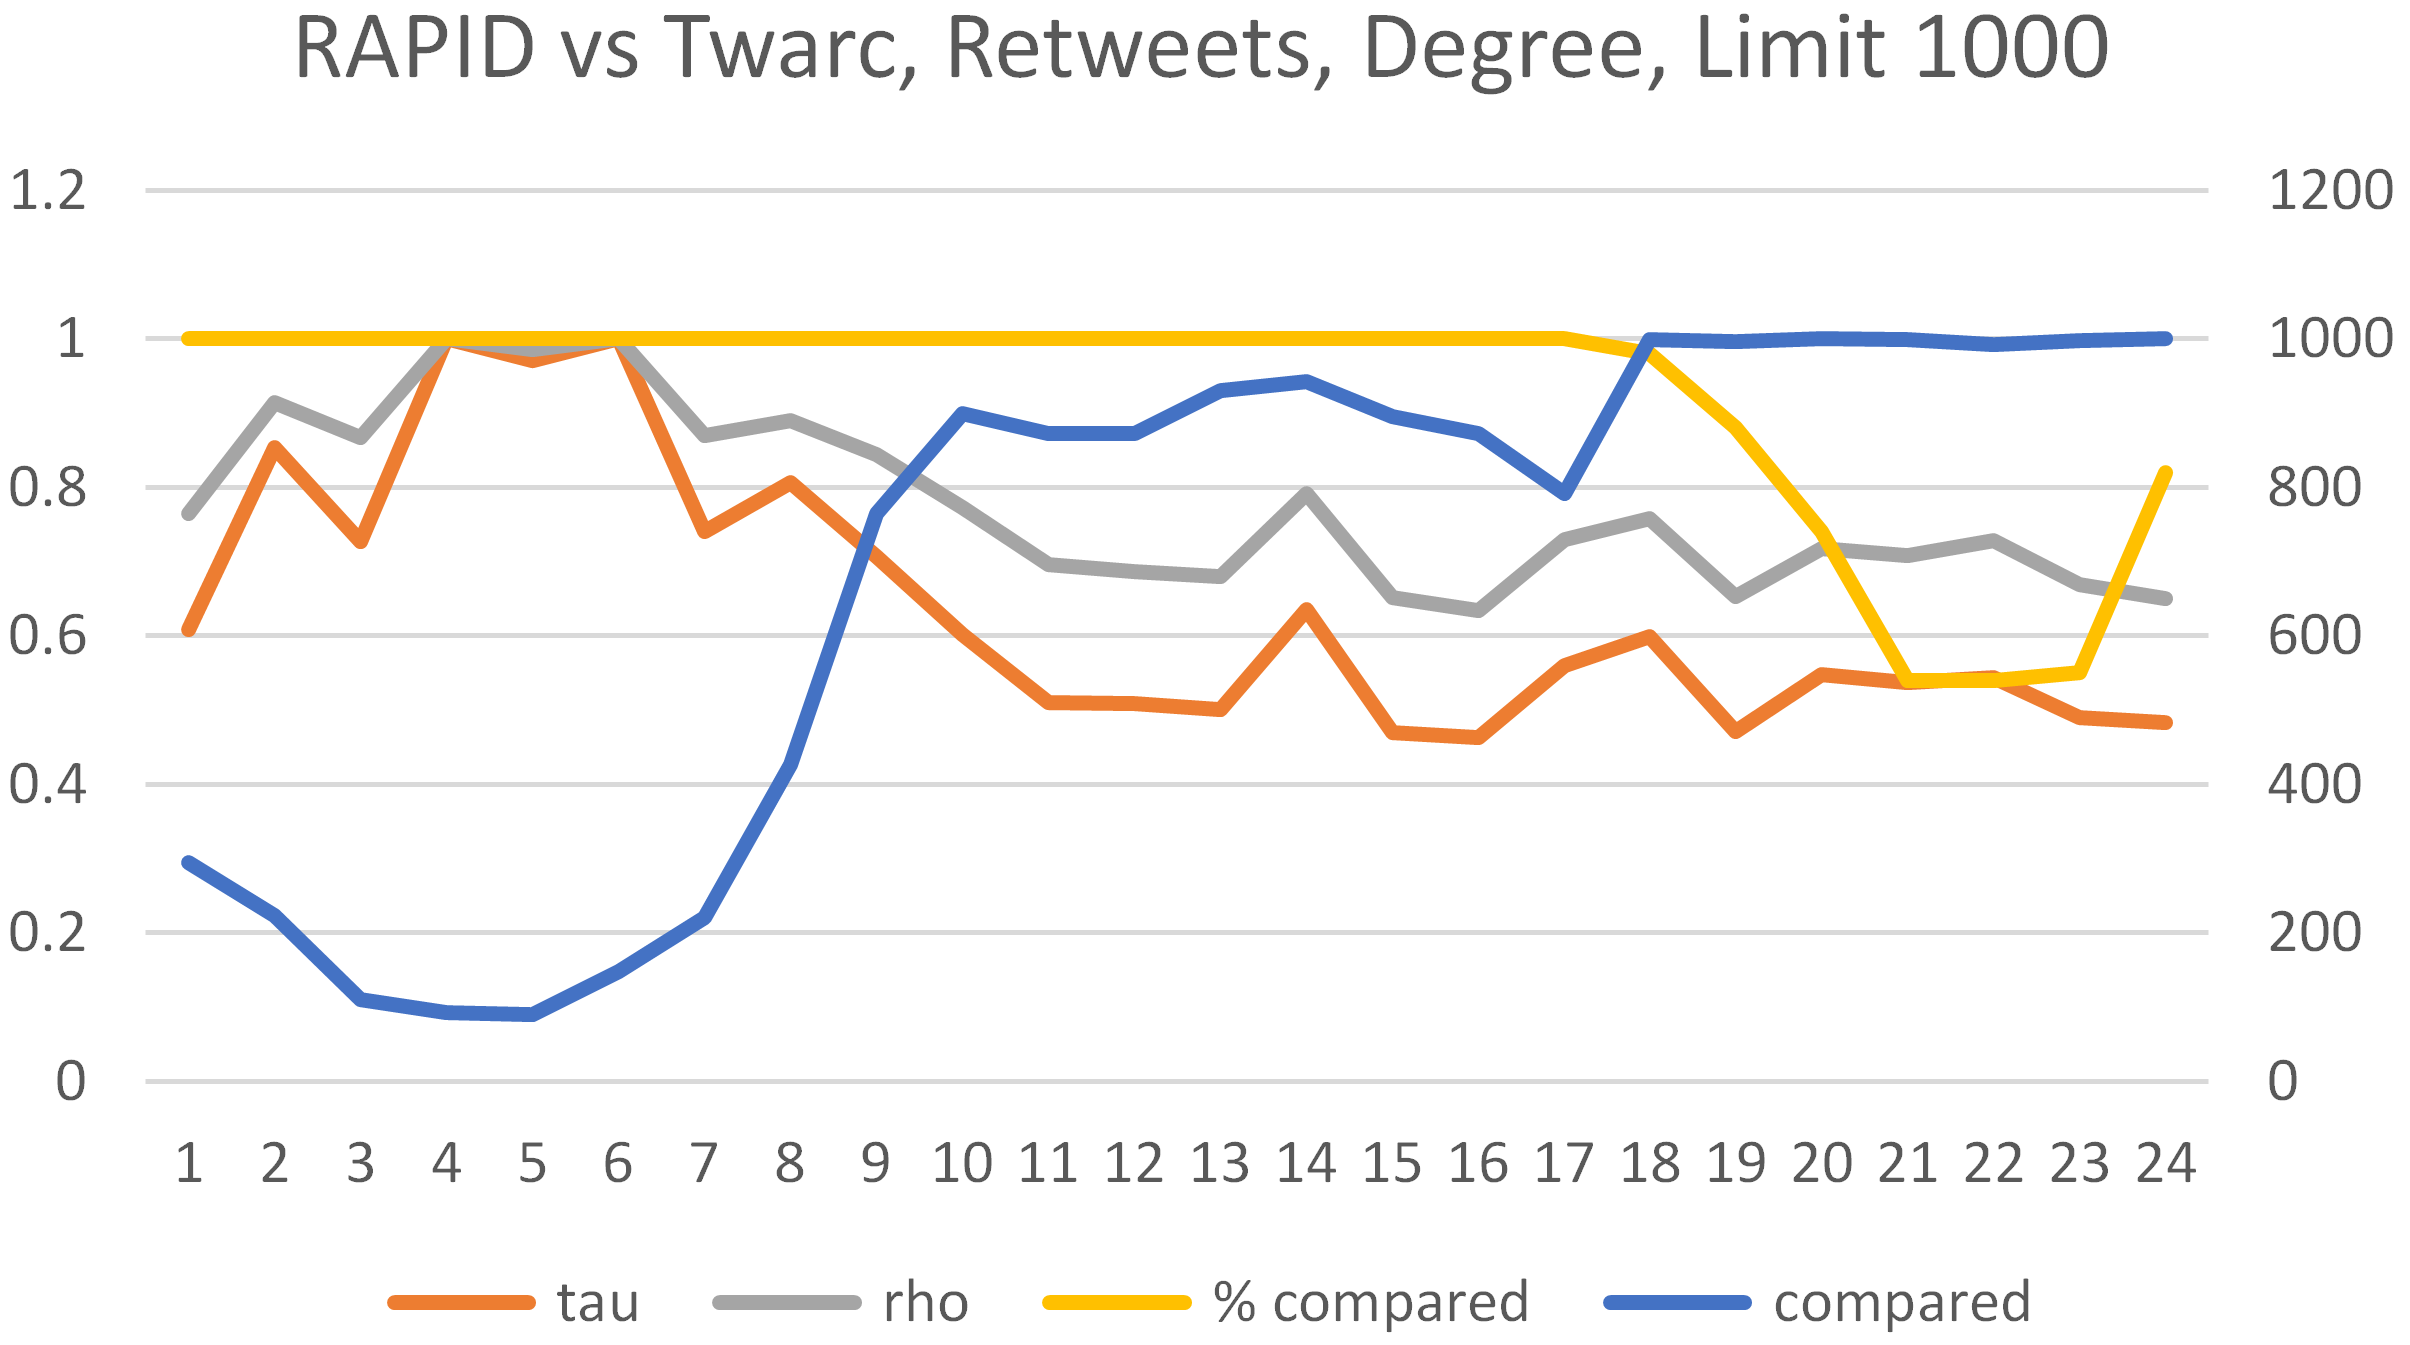}
        \caption{\tiny Retweet/Degree.}
        \label{fig:elec_long_comparison_rt_deg}
    \end{subfigure}

    \bigskip
    \begin{subfigure}[b]{0.3\textwidth}
        \centering
        \includegraphics[scale=0.11]{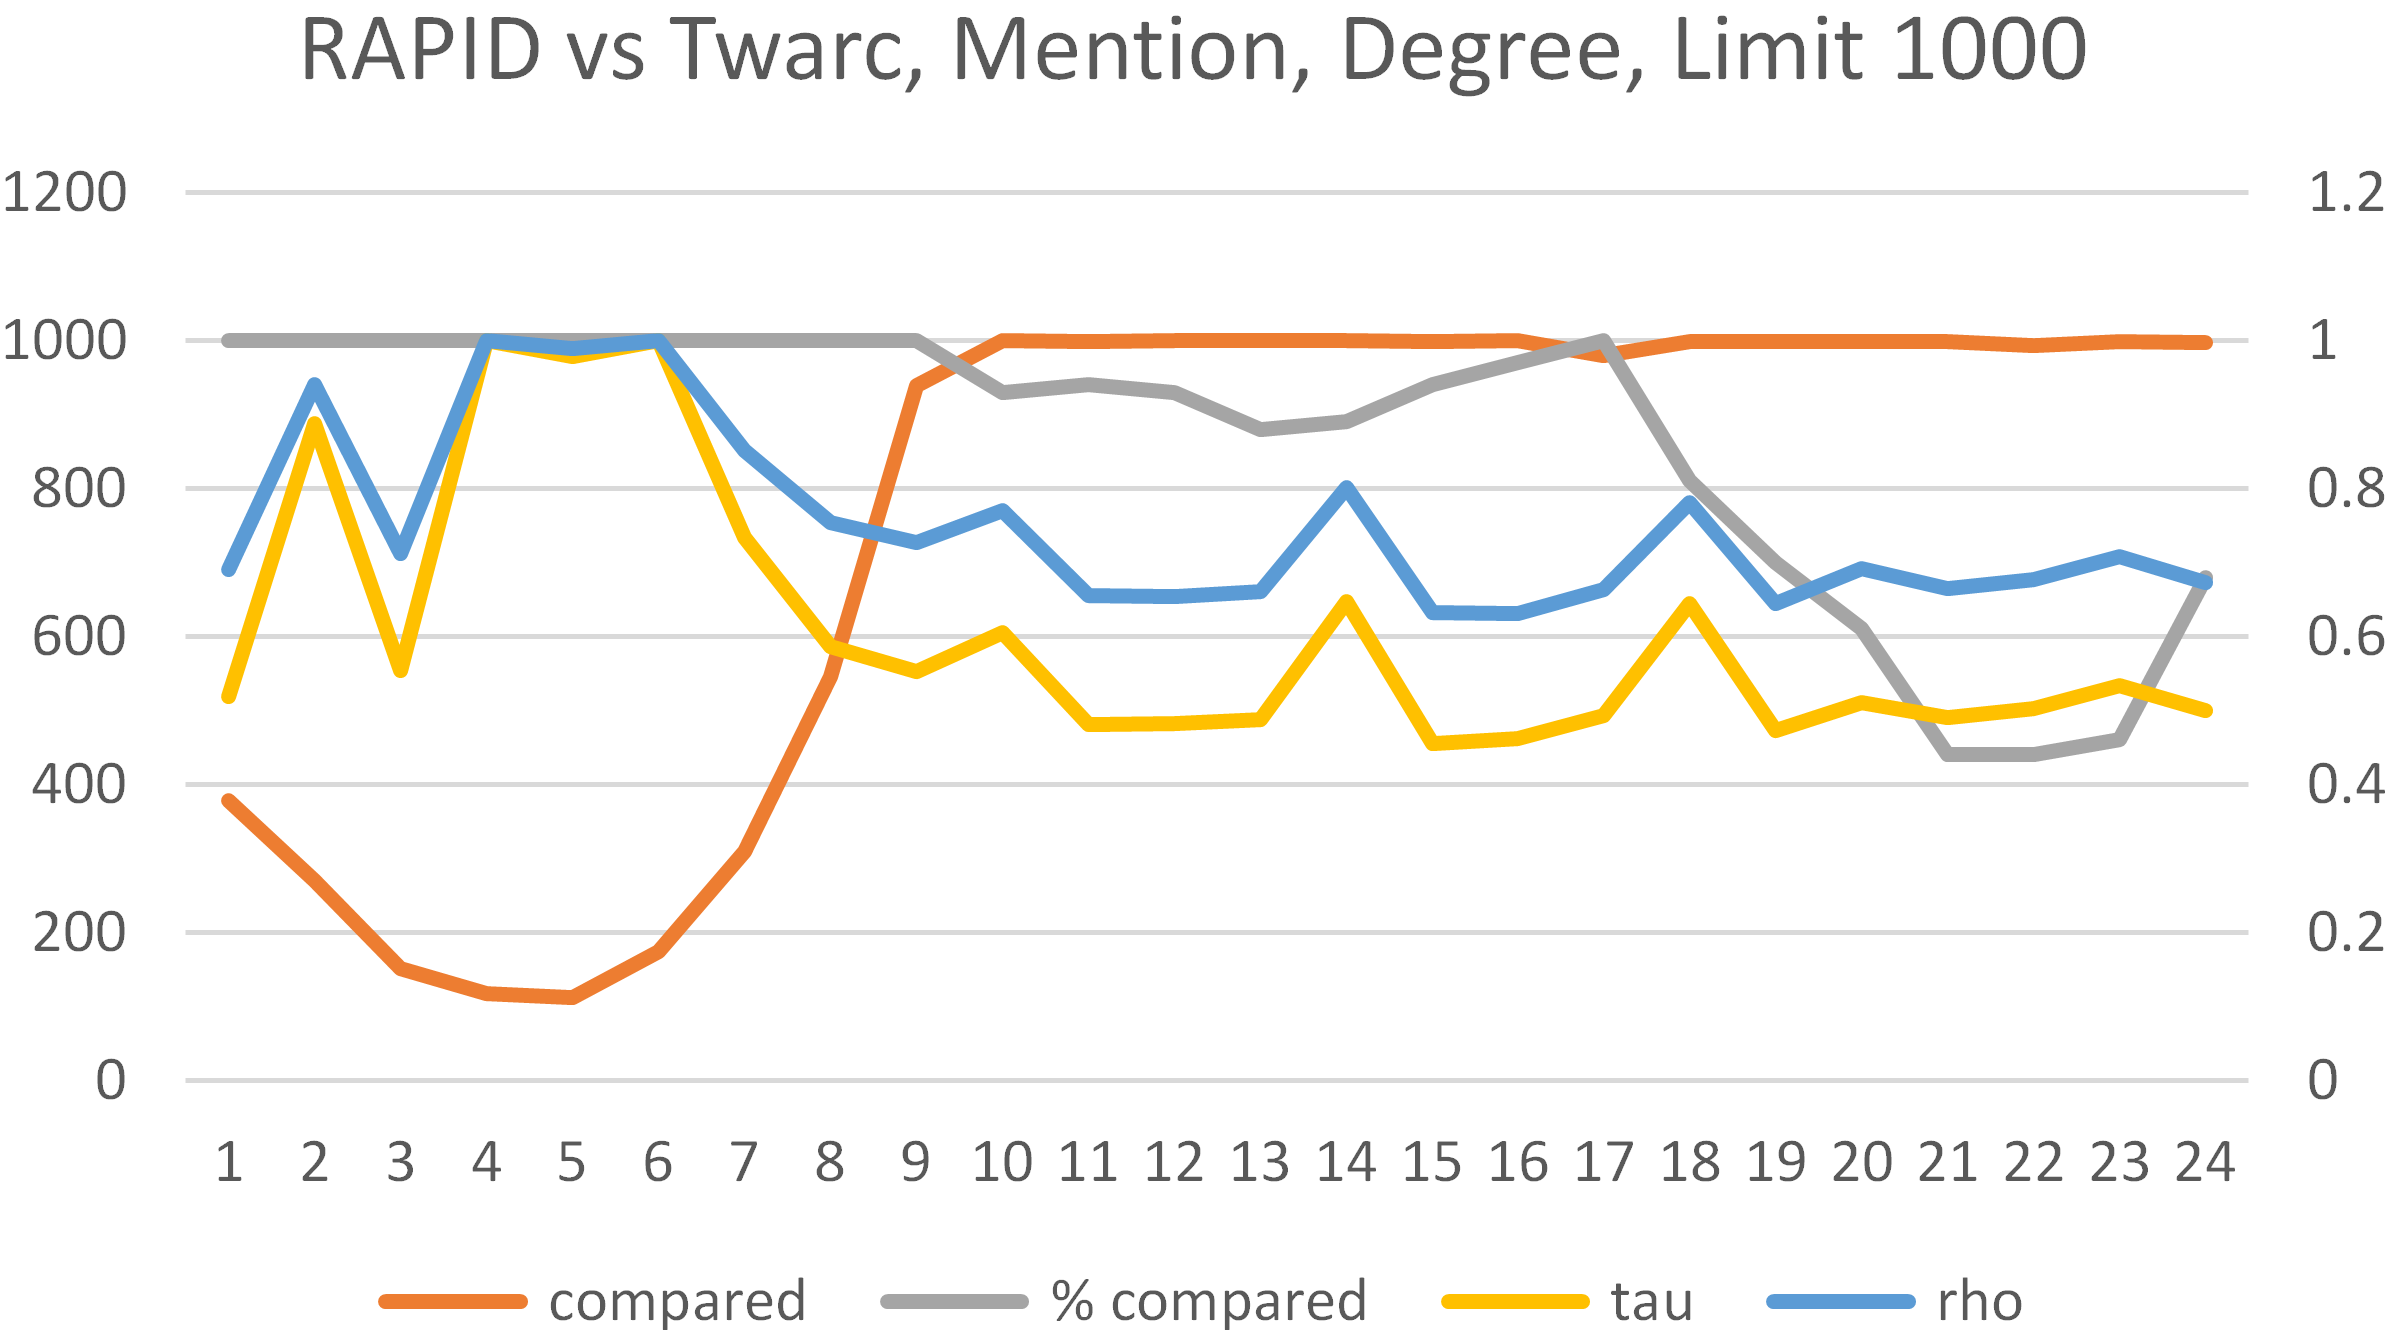}
        \caption{\tiny Mention/Degree.}
        \label{fig:elec_long_comparison_men_deg}
    \end{subfigure}
    \hfill
    \begin{subfigure}[b]{0.3\textwidth}
        \centering
        \includegraphics[scale=0.11]{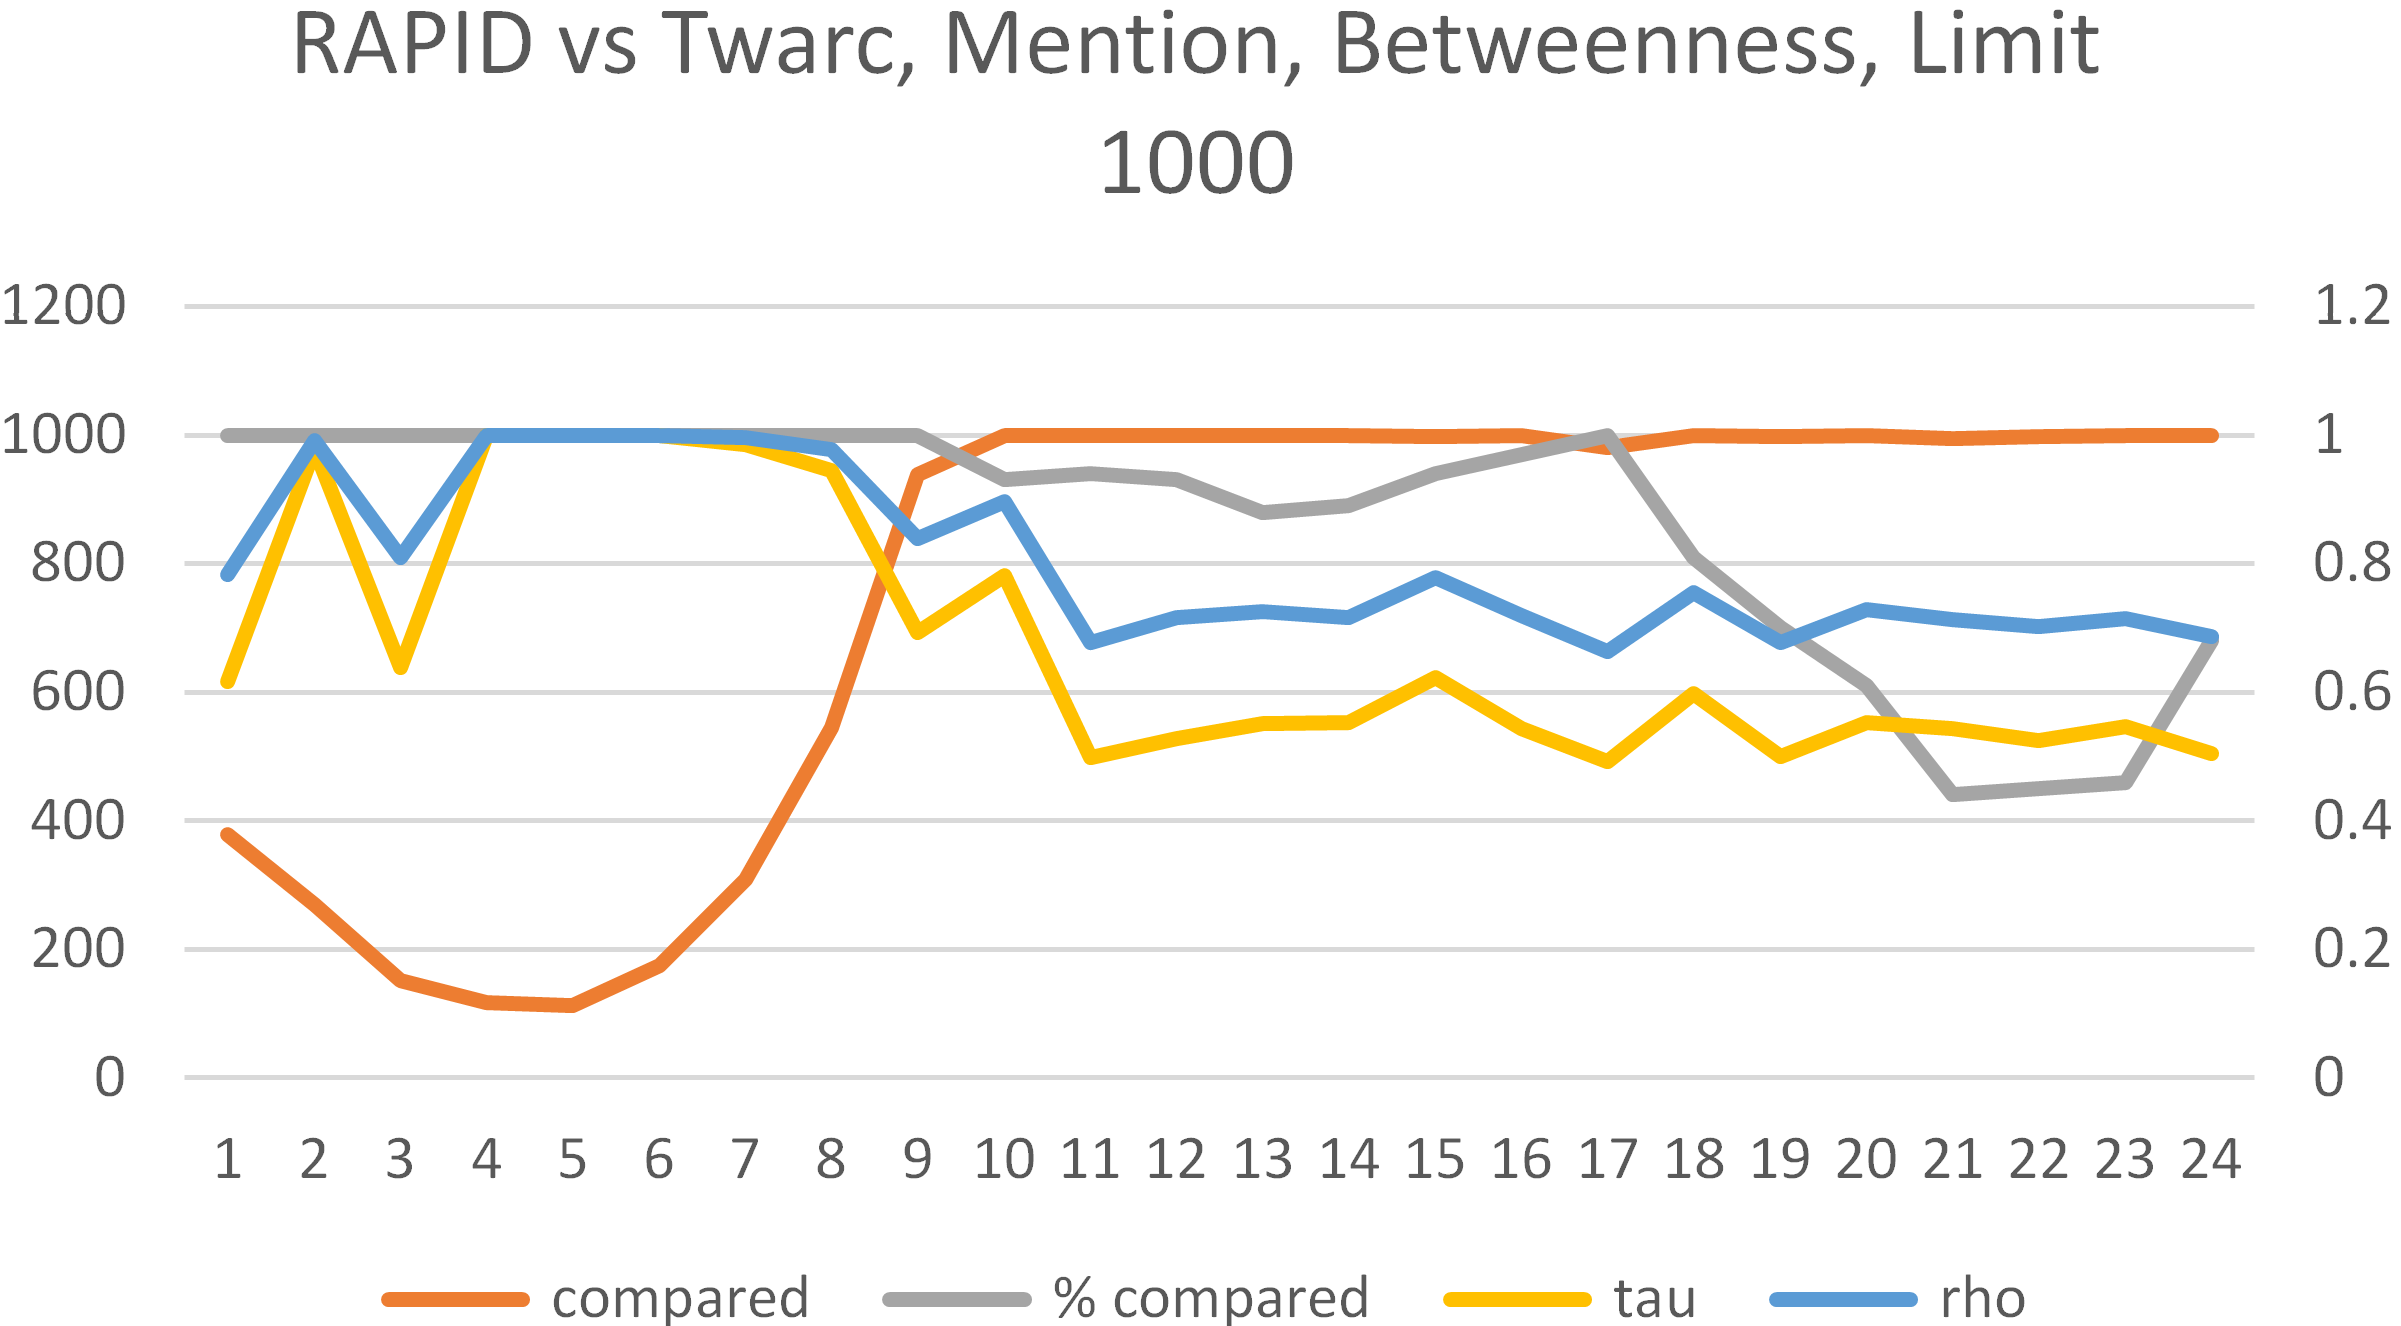}
        \caption{\tiny Mention/Betweenness.}
        \label{fig:elec_long_comparison_men_bet}
    \end{subfigure}
    \hfill
    \begin{subfigure}[b]{0.3\textwidth}
        \centering
        \includegraphics[scale=0.11]{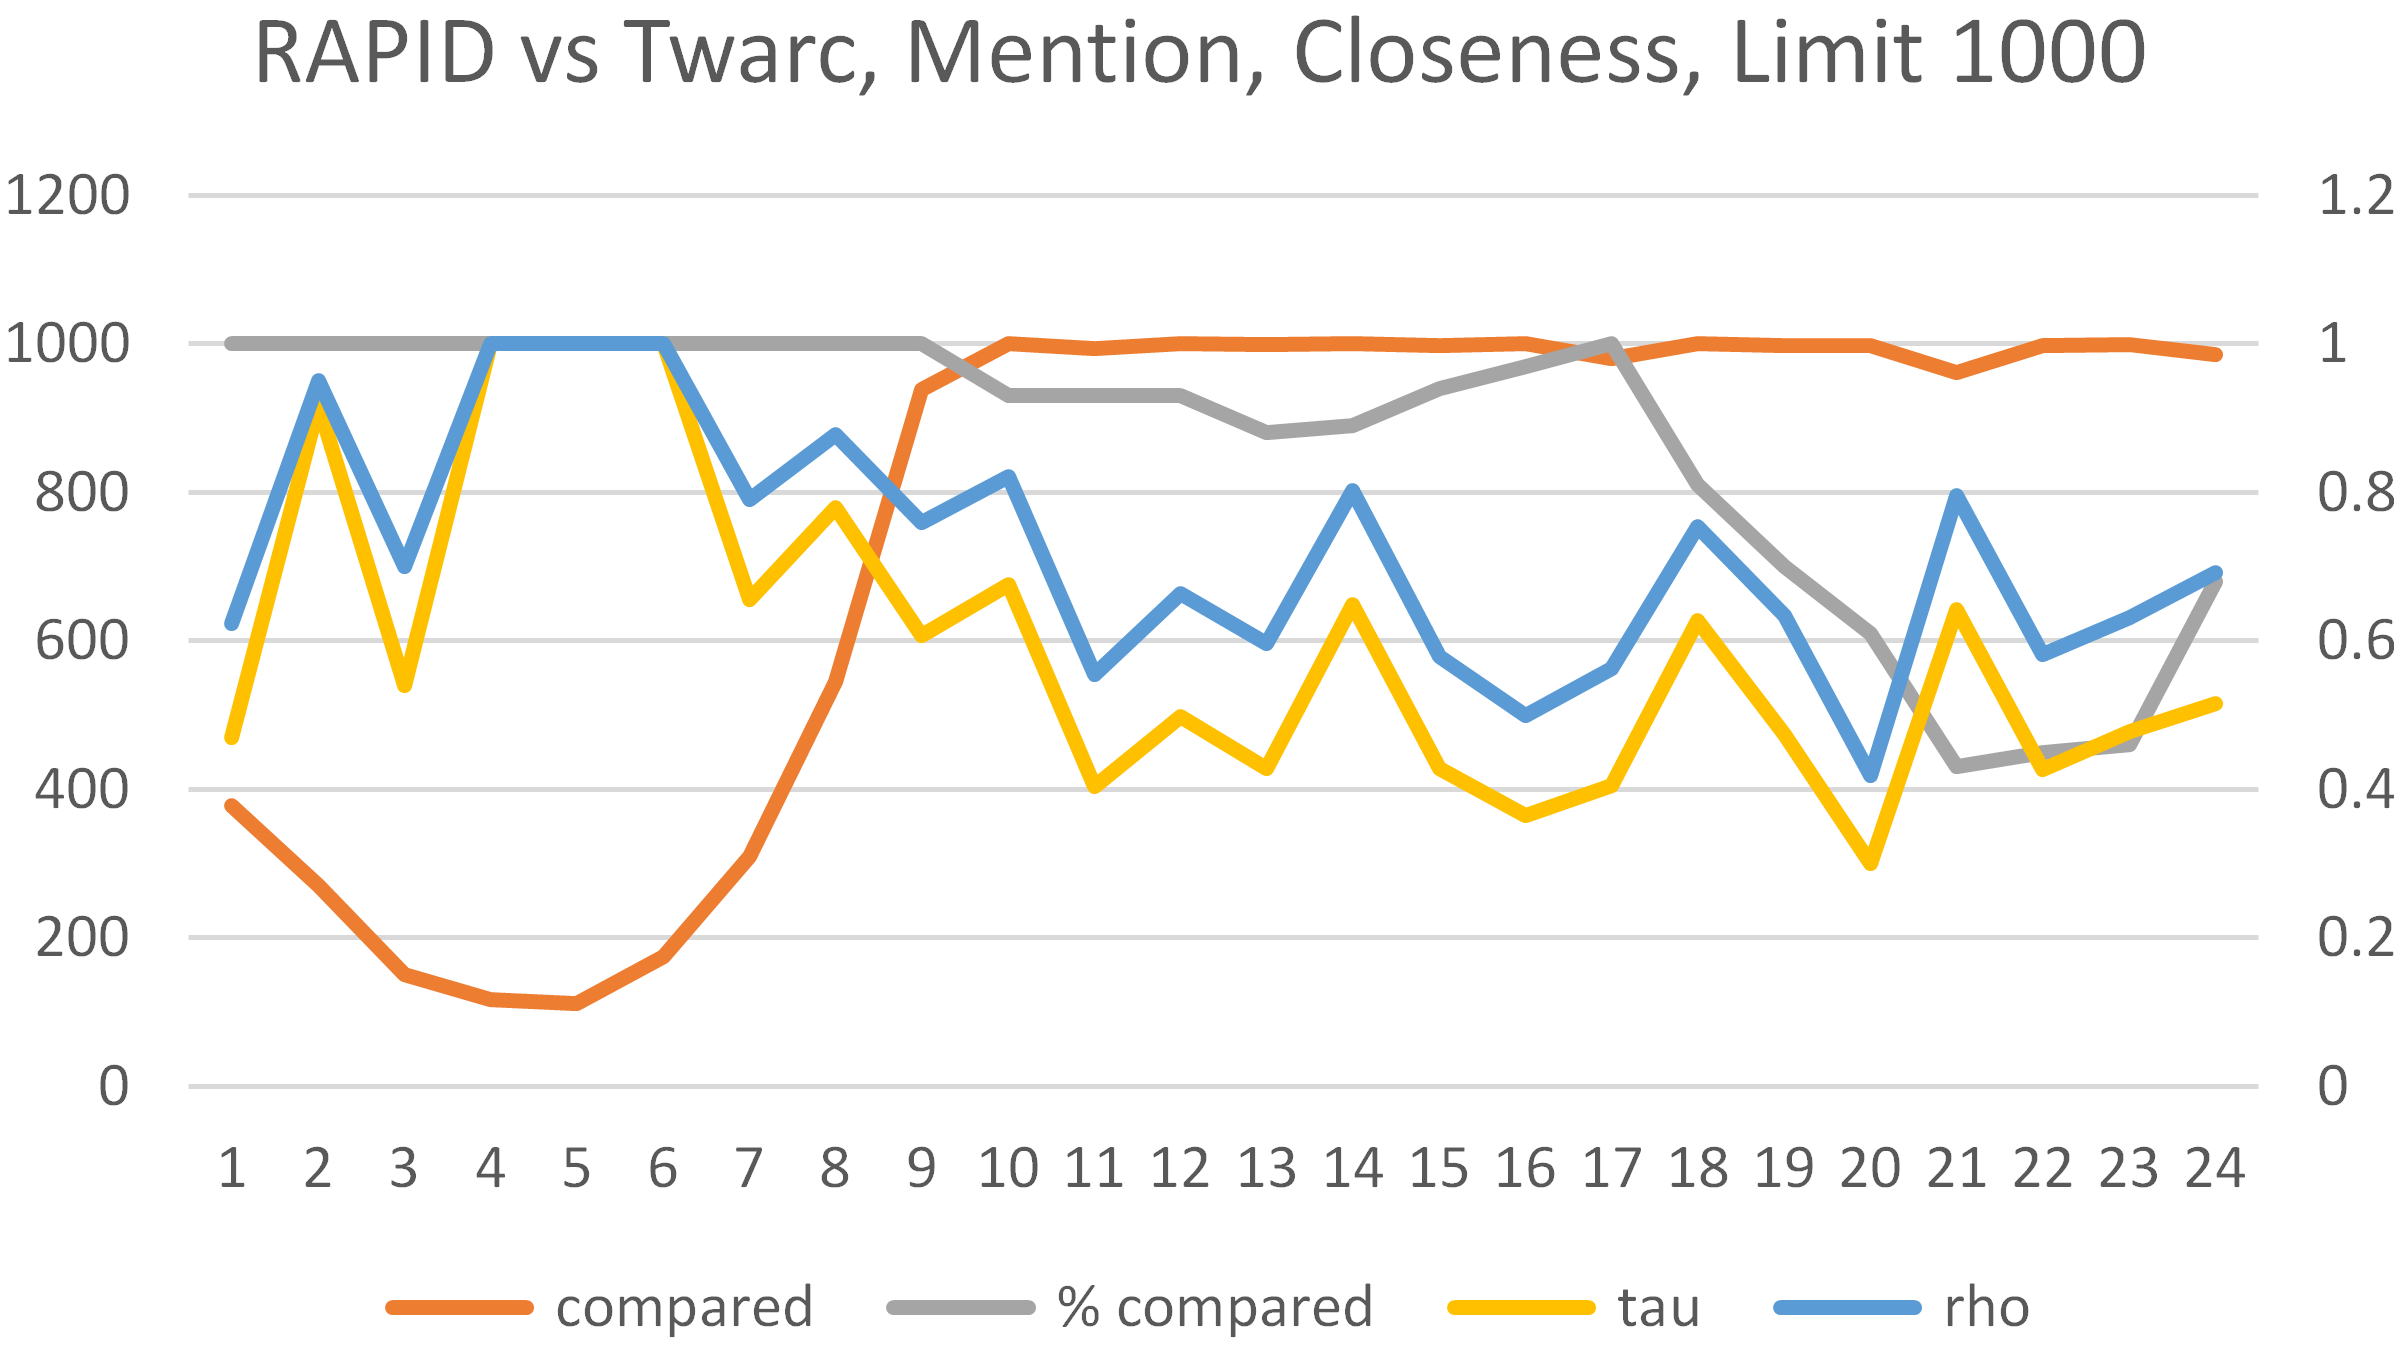}
        \caption{\tiny Mention/Closeness.}
        \label{fig:elec_long_comparison_men_clo}
    \end{subfigure}
    
    \bigskip
    \begin{subfigure}[b]{0.3\textwidth}
        \centering
        \includegraphics[scale=0.11]{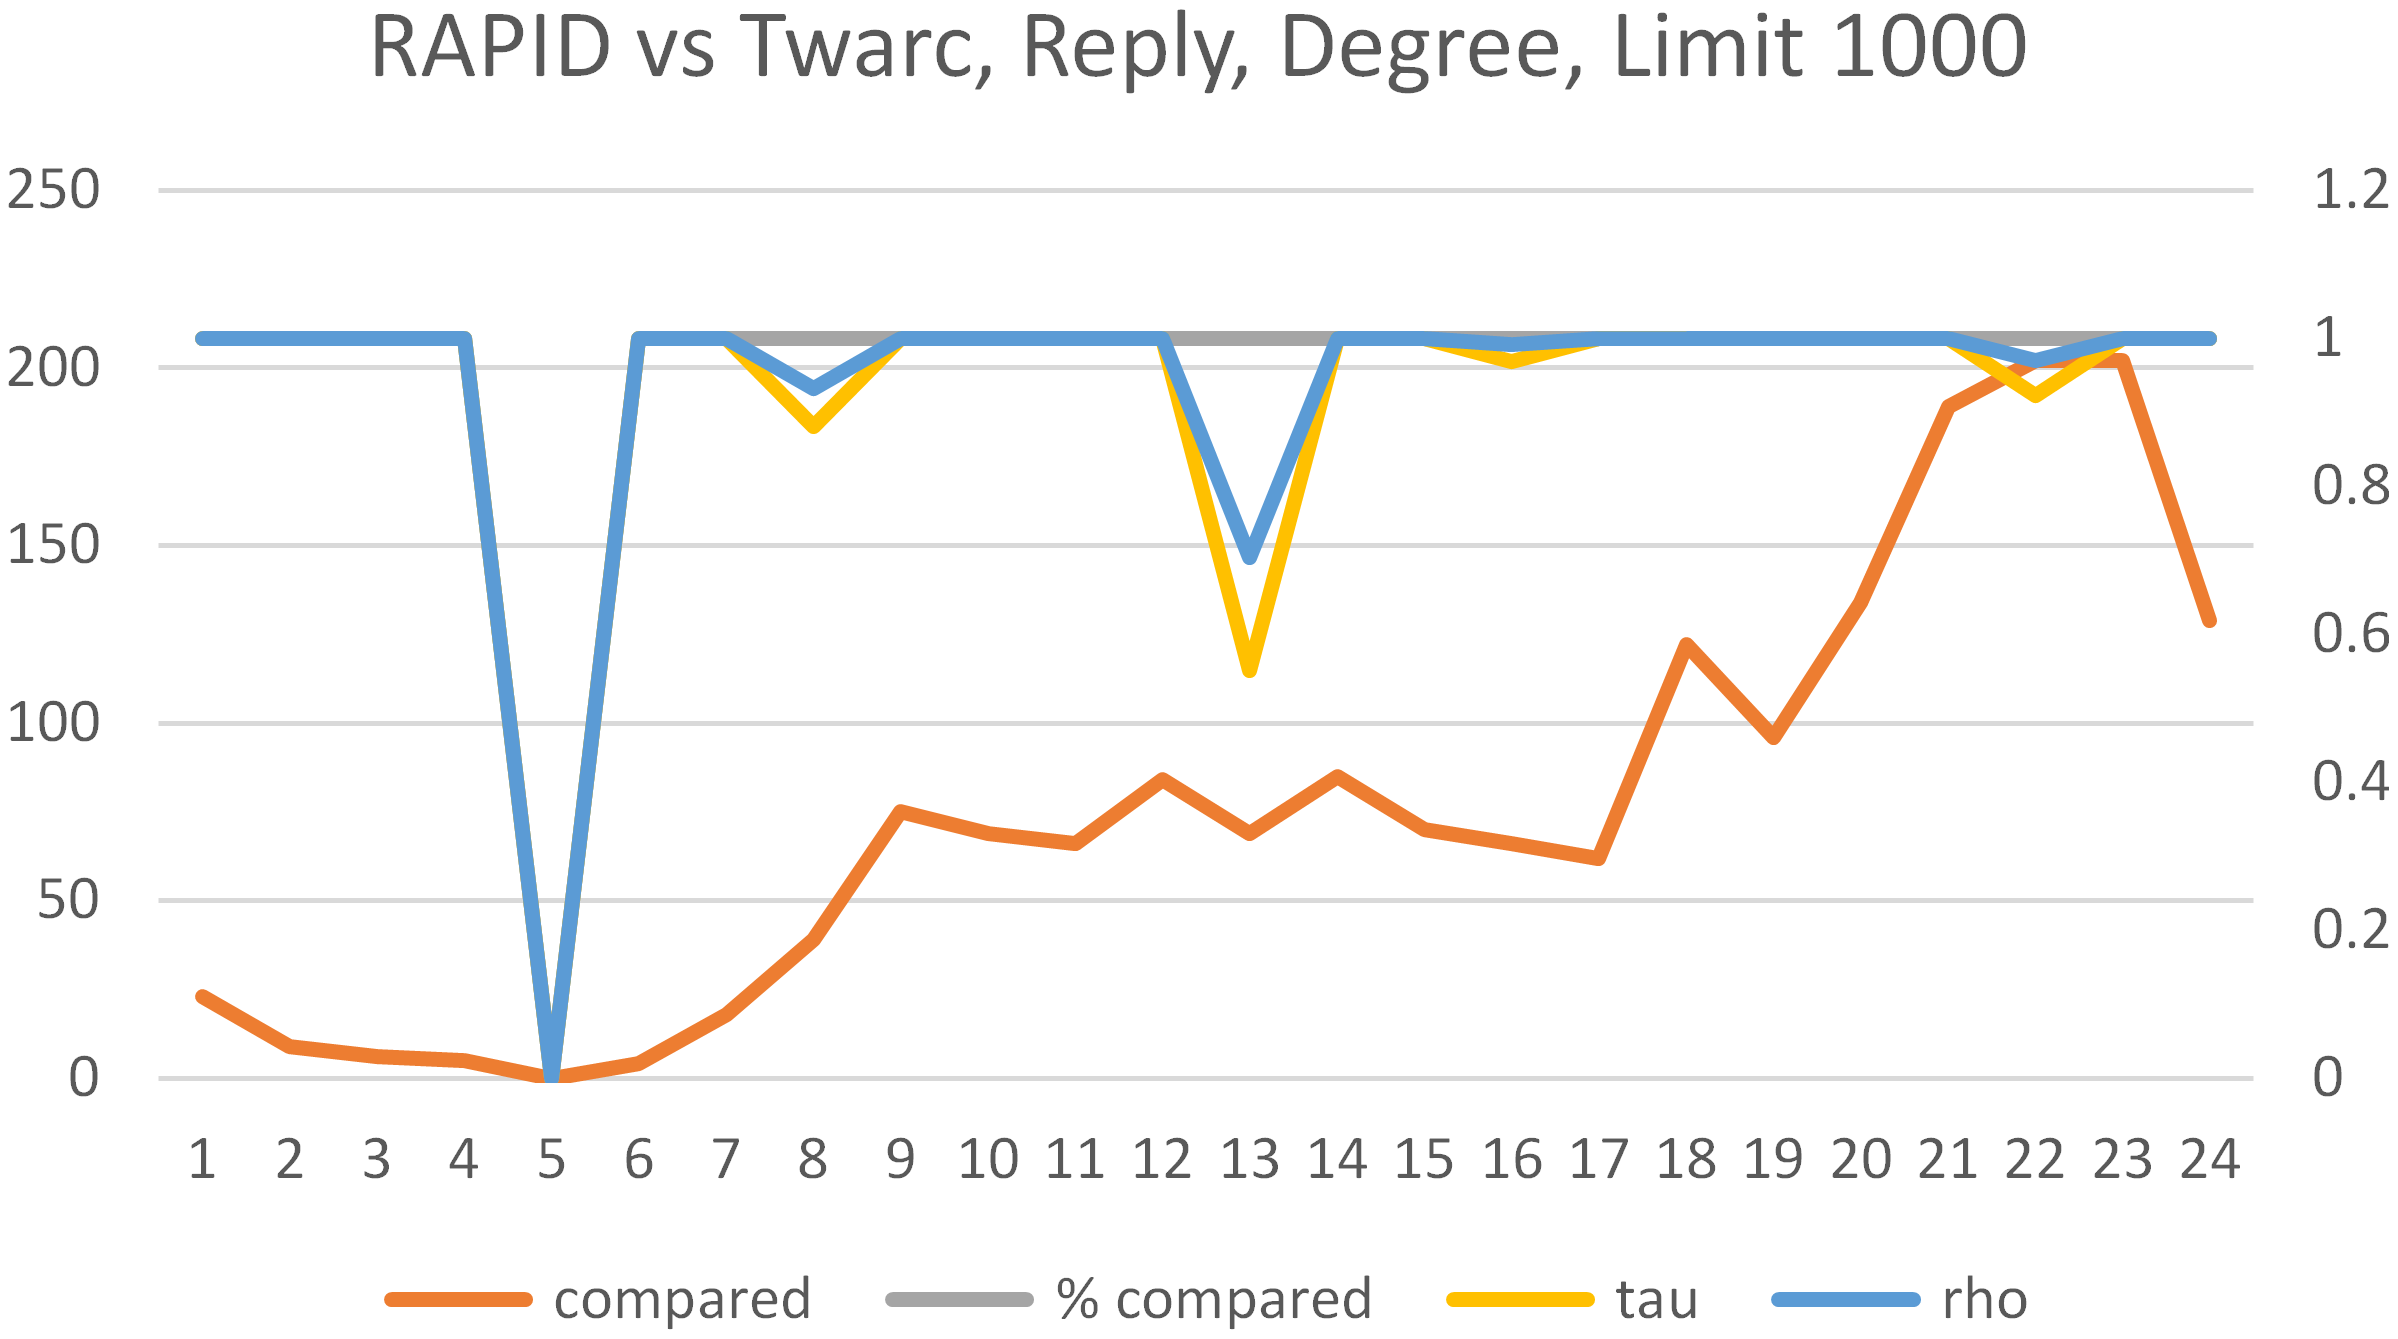}
        \caption{\tiny Reply/Degree.}
        \label{fig:elec_long_comparison_rep_deg}
    \end{subfigure}
    \hfill
    \begin{subfigure}[b]{0.3\textwidth}
        \centering
        \includegraphics[scale=0.11]{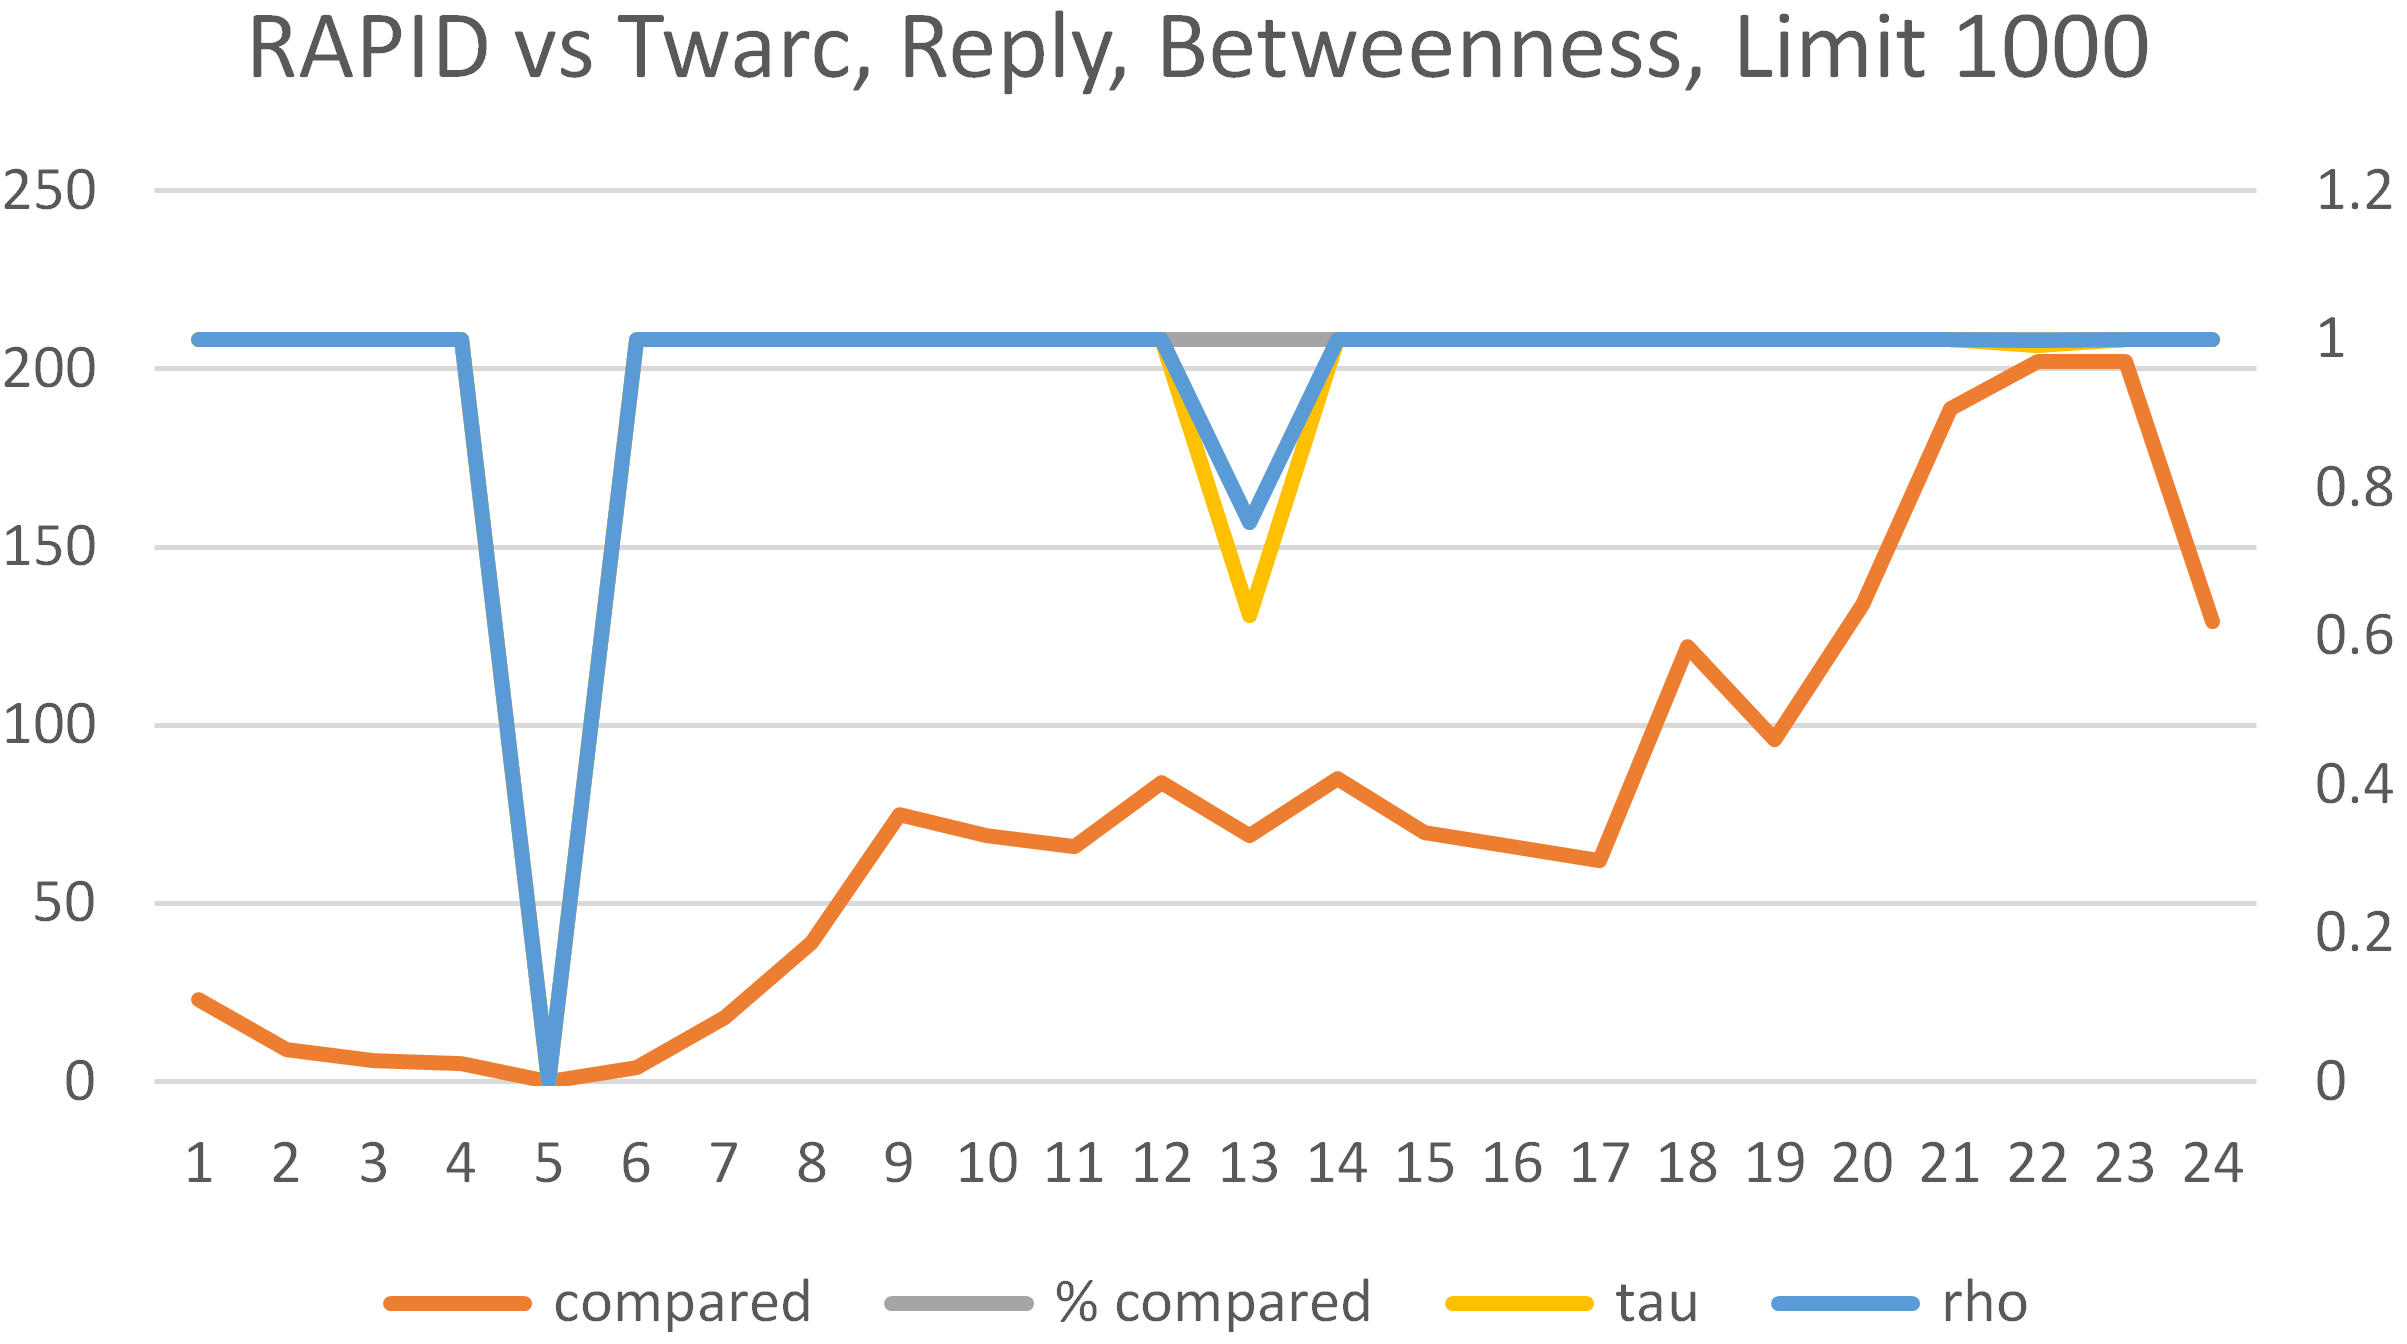}
        \caption{\tiny Reply/Betweenness.}
        \label{fig:elec_long_comparison_rep_bet}
    \end{subfigure}
    \hfill
    \begin{subfigure}[b]{0.3\textwidth}
        \centering
        \includegraphics[scale=0.11]{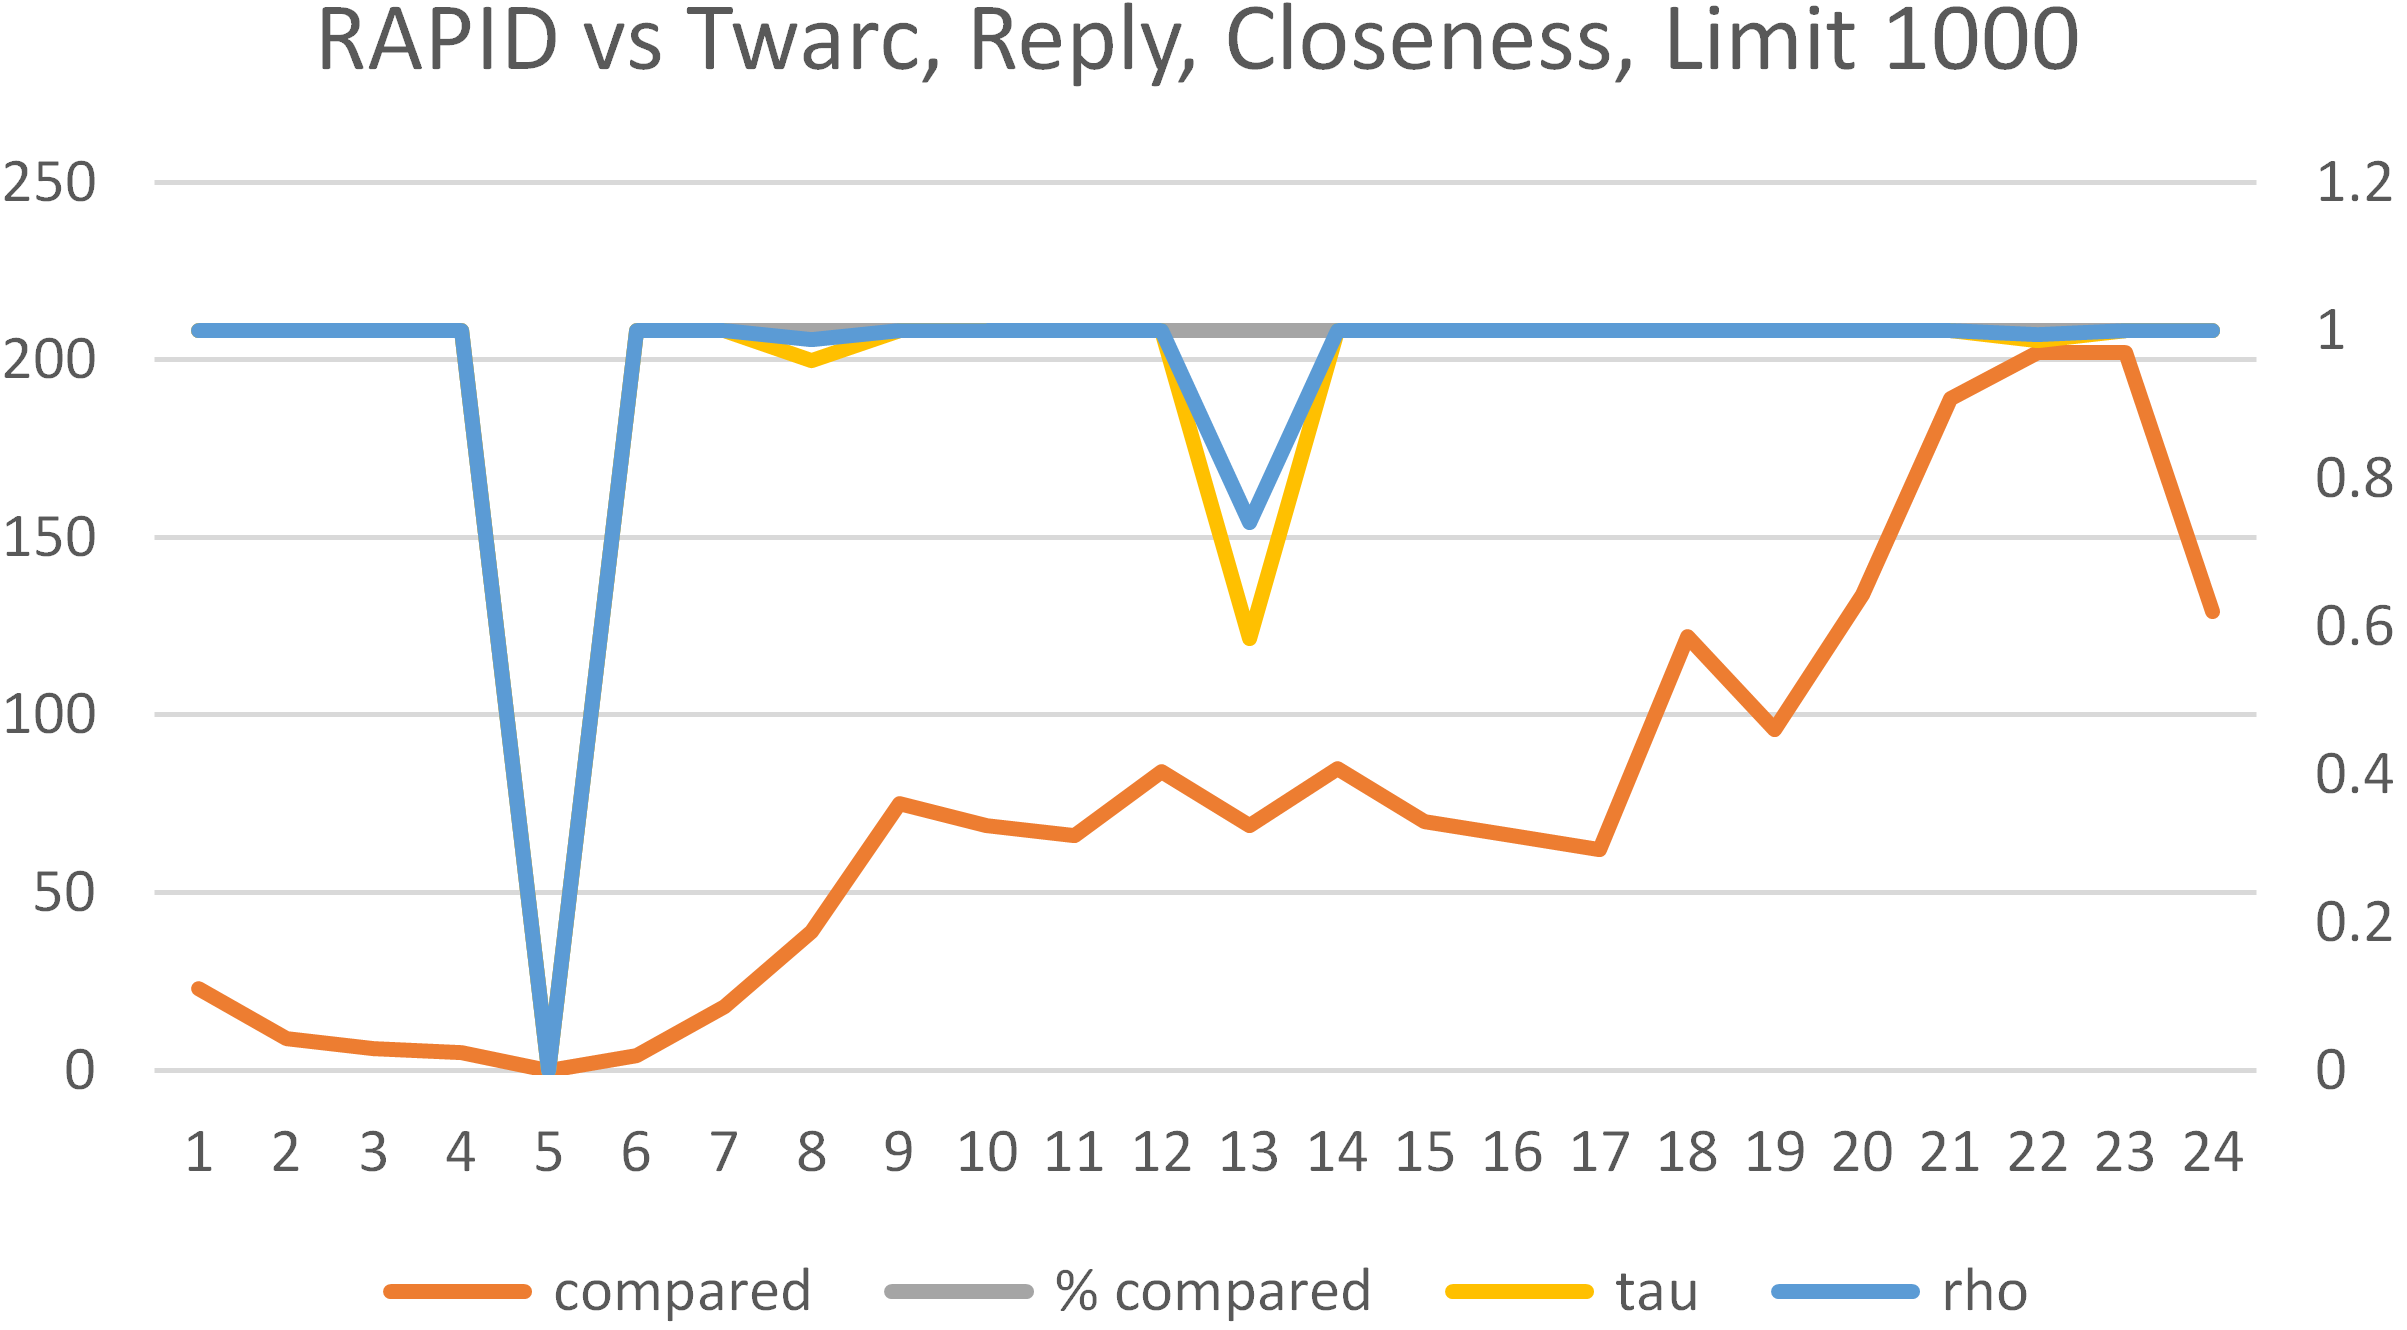}
        \caption{\tiny Reply/Closeness.}
        \label{fig:elec_long_comparison_rep_clo}
    \end{subfigure}

    \caption{Longitudinal centrality ranking comparisons from the RAPID and Twarc datasets of the ``Election Day'' collections using Kendall Tau scores and Spearman's Coefficients.}
    \label{fig:elec_long_comparison}
\end{figure}

For all charts in Figure \ref{fig:elec_long_comparison}, the ``compared'' series refers to the number of ranked nodes actually compared. Each bucket may be of a different size, given the activity in the particular hour it represents, and so it is necessary to offer the length of ranked lists compared as well as how large a proportion this represents -- the ``\% compared'' series refers to the number compared as a proportion of the smaller of the lists (either from the corresponding RAPID or Twarc datasets) for that hour. It is clear that the early hours of the dataset refer to the night prior to the election day itself, and so there is a dip in the number of comparisons, and the proportion of those compared is relatively high. Later in the collections the proportion dips as more authors are considered and the rankings change. The tau and rho metrics remain relatively similar and proportional throughout. The reply network figures are much smaller, due to the observably smaller number of replies in the datasets.

DCW: I DON'T KNOW ENOUGH ABOUT HOW KENDALL TAU AND SPEARMAN'S COEFFICIENTS WORK TO SAY WHY THEIR VALUES ARE SIMILAR BUT NOT IDENTICAL. 

To consider the effect of introducing new posts and corresponding authors into the collection over time, we also present the results as they accumulate in Figure \ref{fig:elec_long_comparison_cumulative}. Due to the upper limit of 1000 nodes to consider, both the retweet and mention graphs cap at about seven or eight hours, and the proportion of nodes compared drops steadily from this point (as more authors are accumulated). What is notable is that the proportion of nodes matched starts and stays high until that point, meaning the same nodes are appearing in both lists, which indicates a degree of alignment between the datasets. The similarity metrics indicate that the nodes appear in different orders, however, though, again, $\tau$ and $\rho$ appear to be consistently correlated. The artifacts that occur in the similarity scores aroudn the 17th or 18th hour correspond closely with the closing of the polls, and may be indicative of a spike of new activity from authors - the number of authors does not spike, but their ordering changes markedly, which would be indicative of a change in behaviour.

\begin{figure}[t!]
    \centering
    \begin{subfigure}[b]{0.3\textwidth}
        \centering
        \includegraphics[scale=0.11]{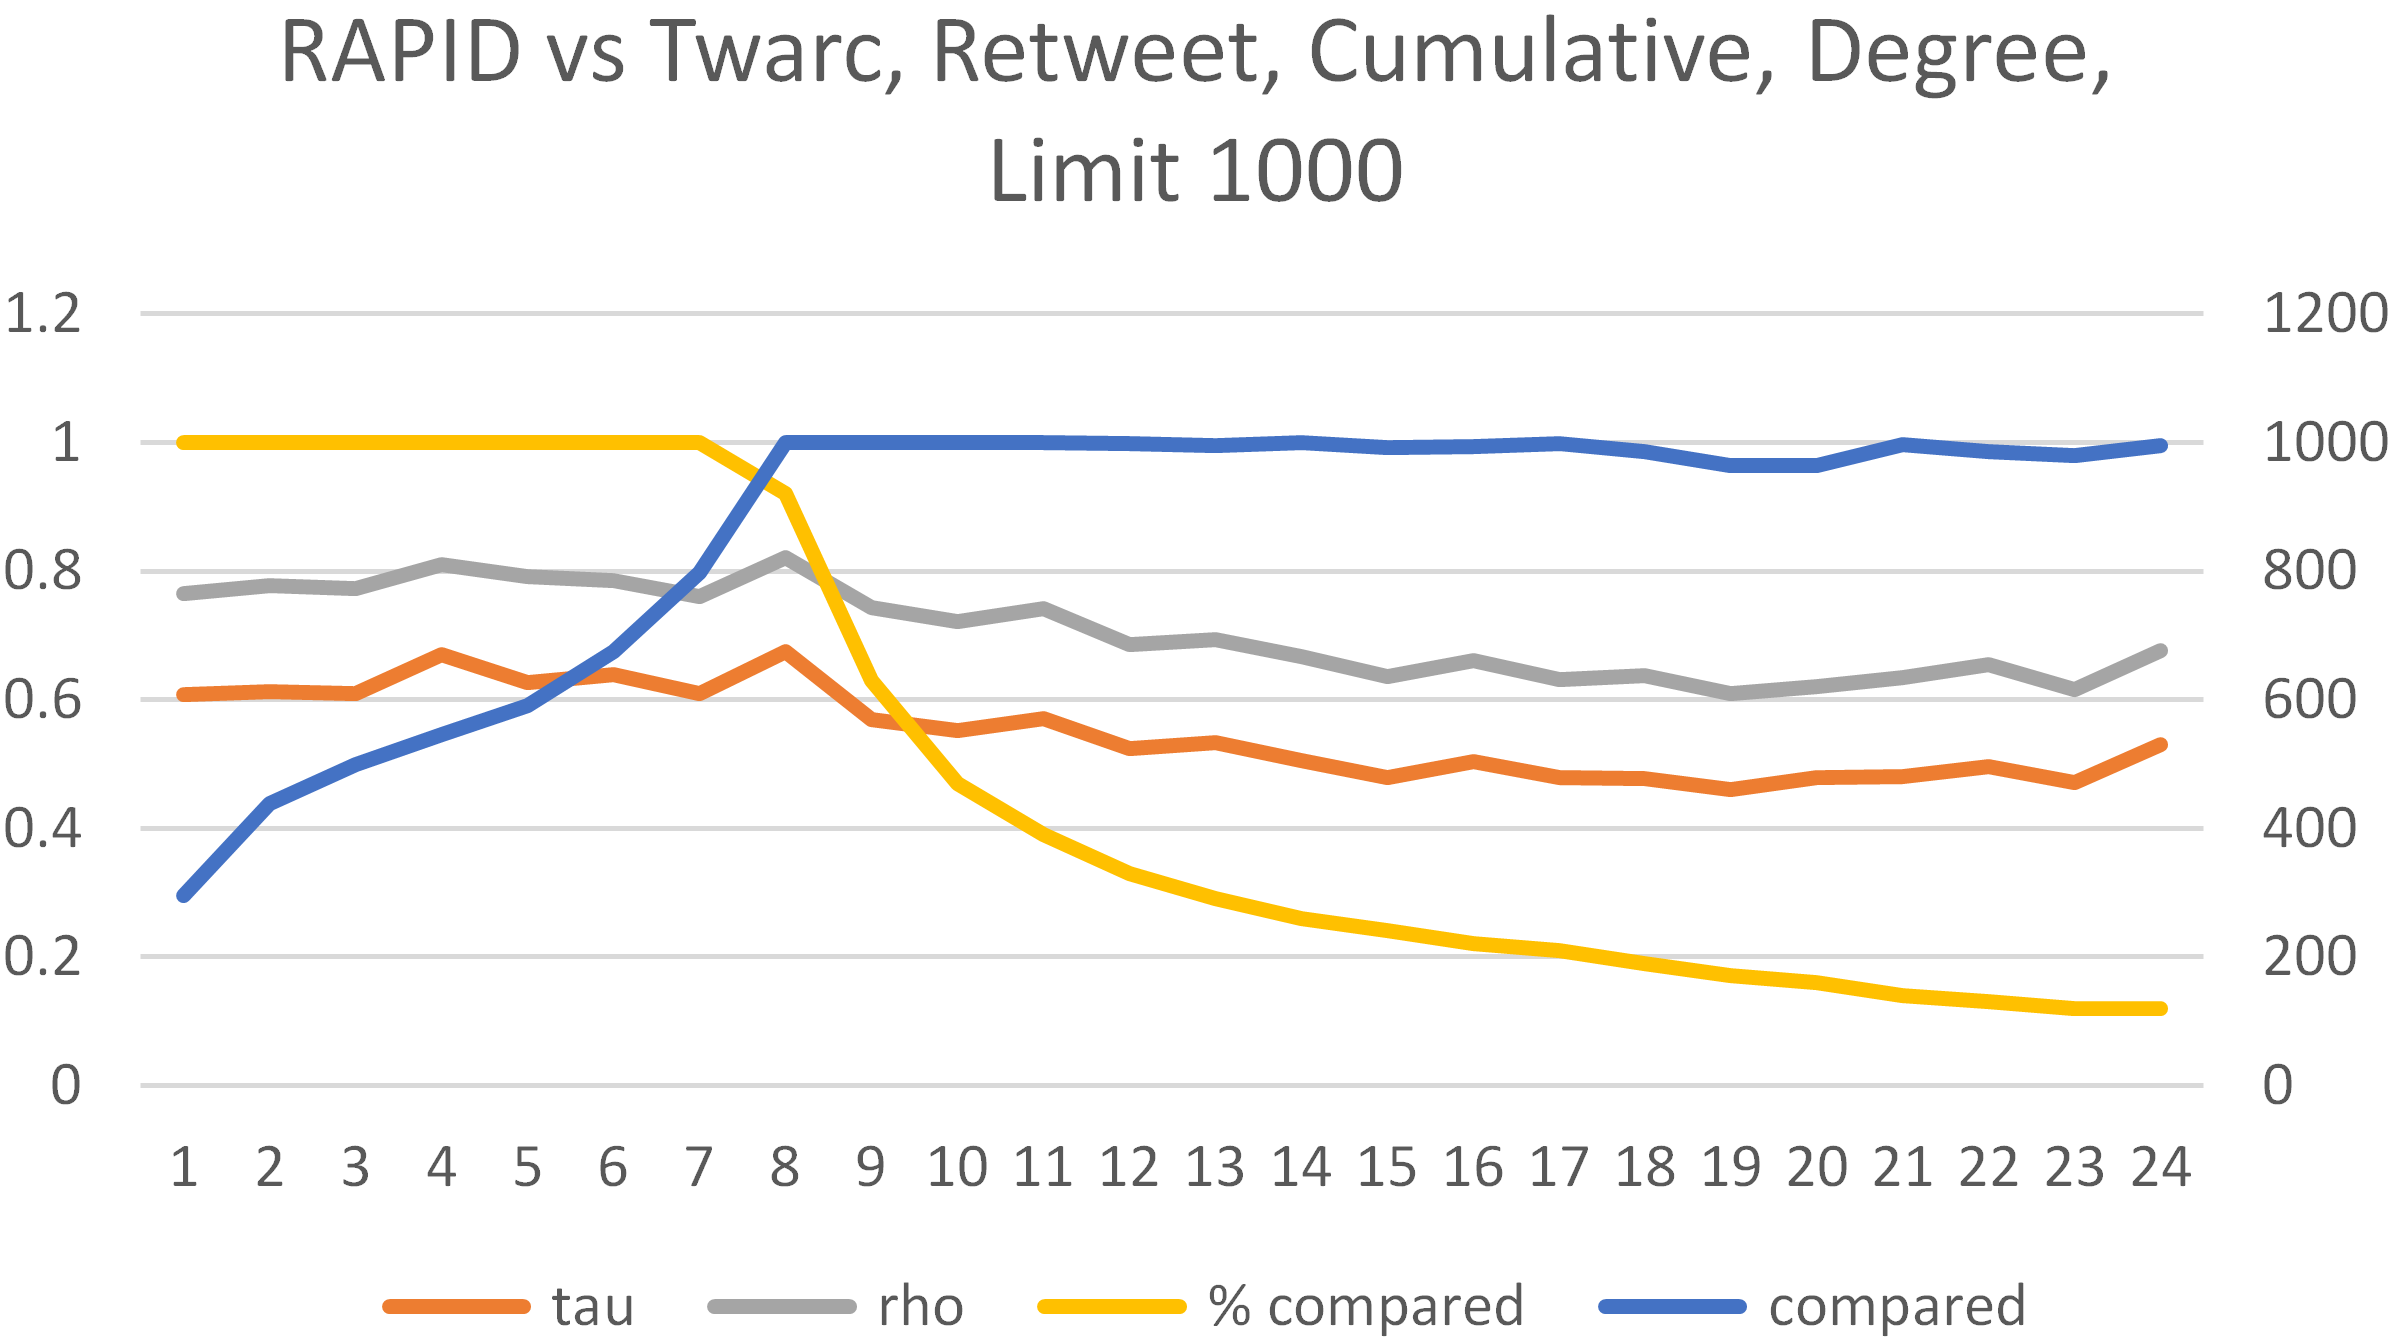}
        \caption{\tiny Retweet/Degree.}
        \label{fig:elec_long_comparison_cumulative_rt_deg}
    \end{subfigure}

    \bigskip
    \begin{subfigure}[b]{0.3\textwidth}
        \centering
        \includegraphics[scale=0.11]{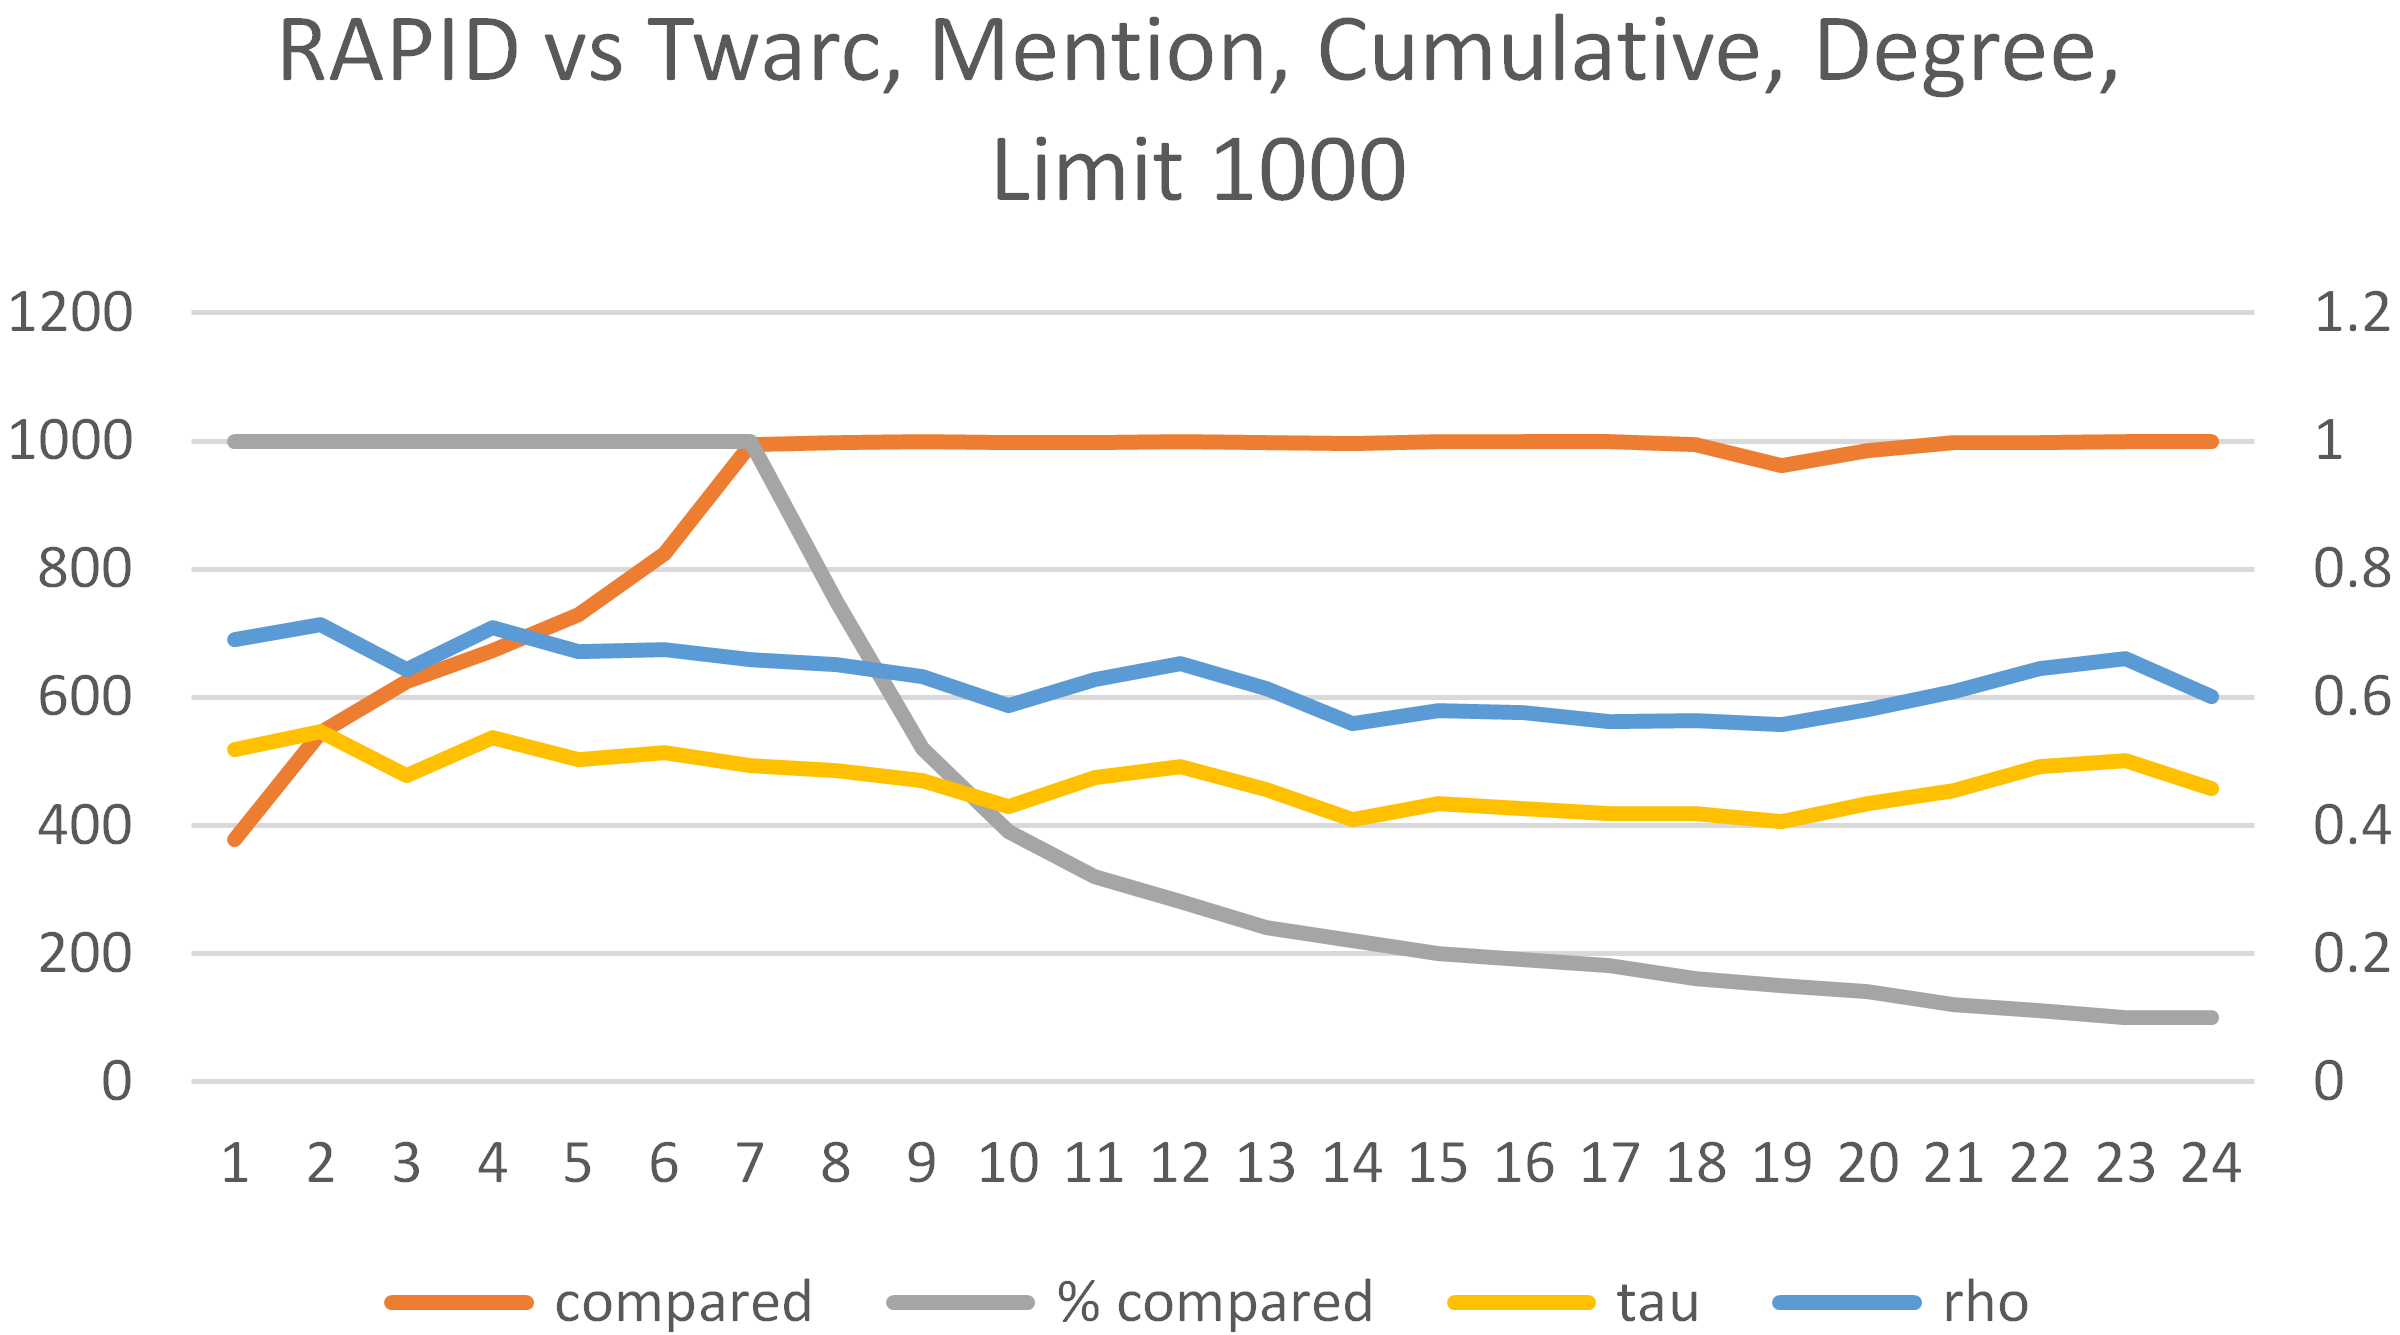}
        \caption{\tiny Mention/Degree.}
        \label{fig:elec_long_comparison_cumulative_men_deg}
    \end{subfigure}
    \hfill
    \begin{subfigure}[b]{0.3\textwidth}
        \centering
        \includegraphics[scale=0.11]{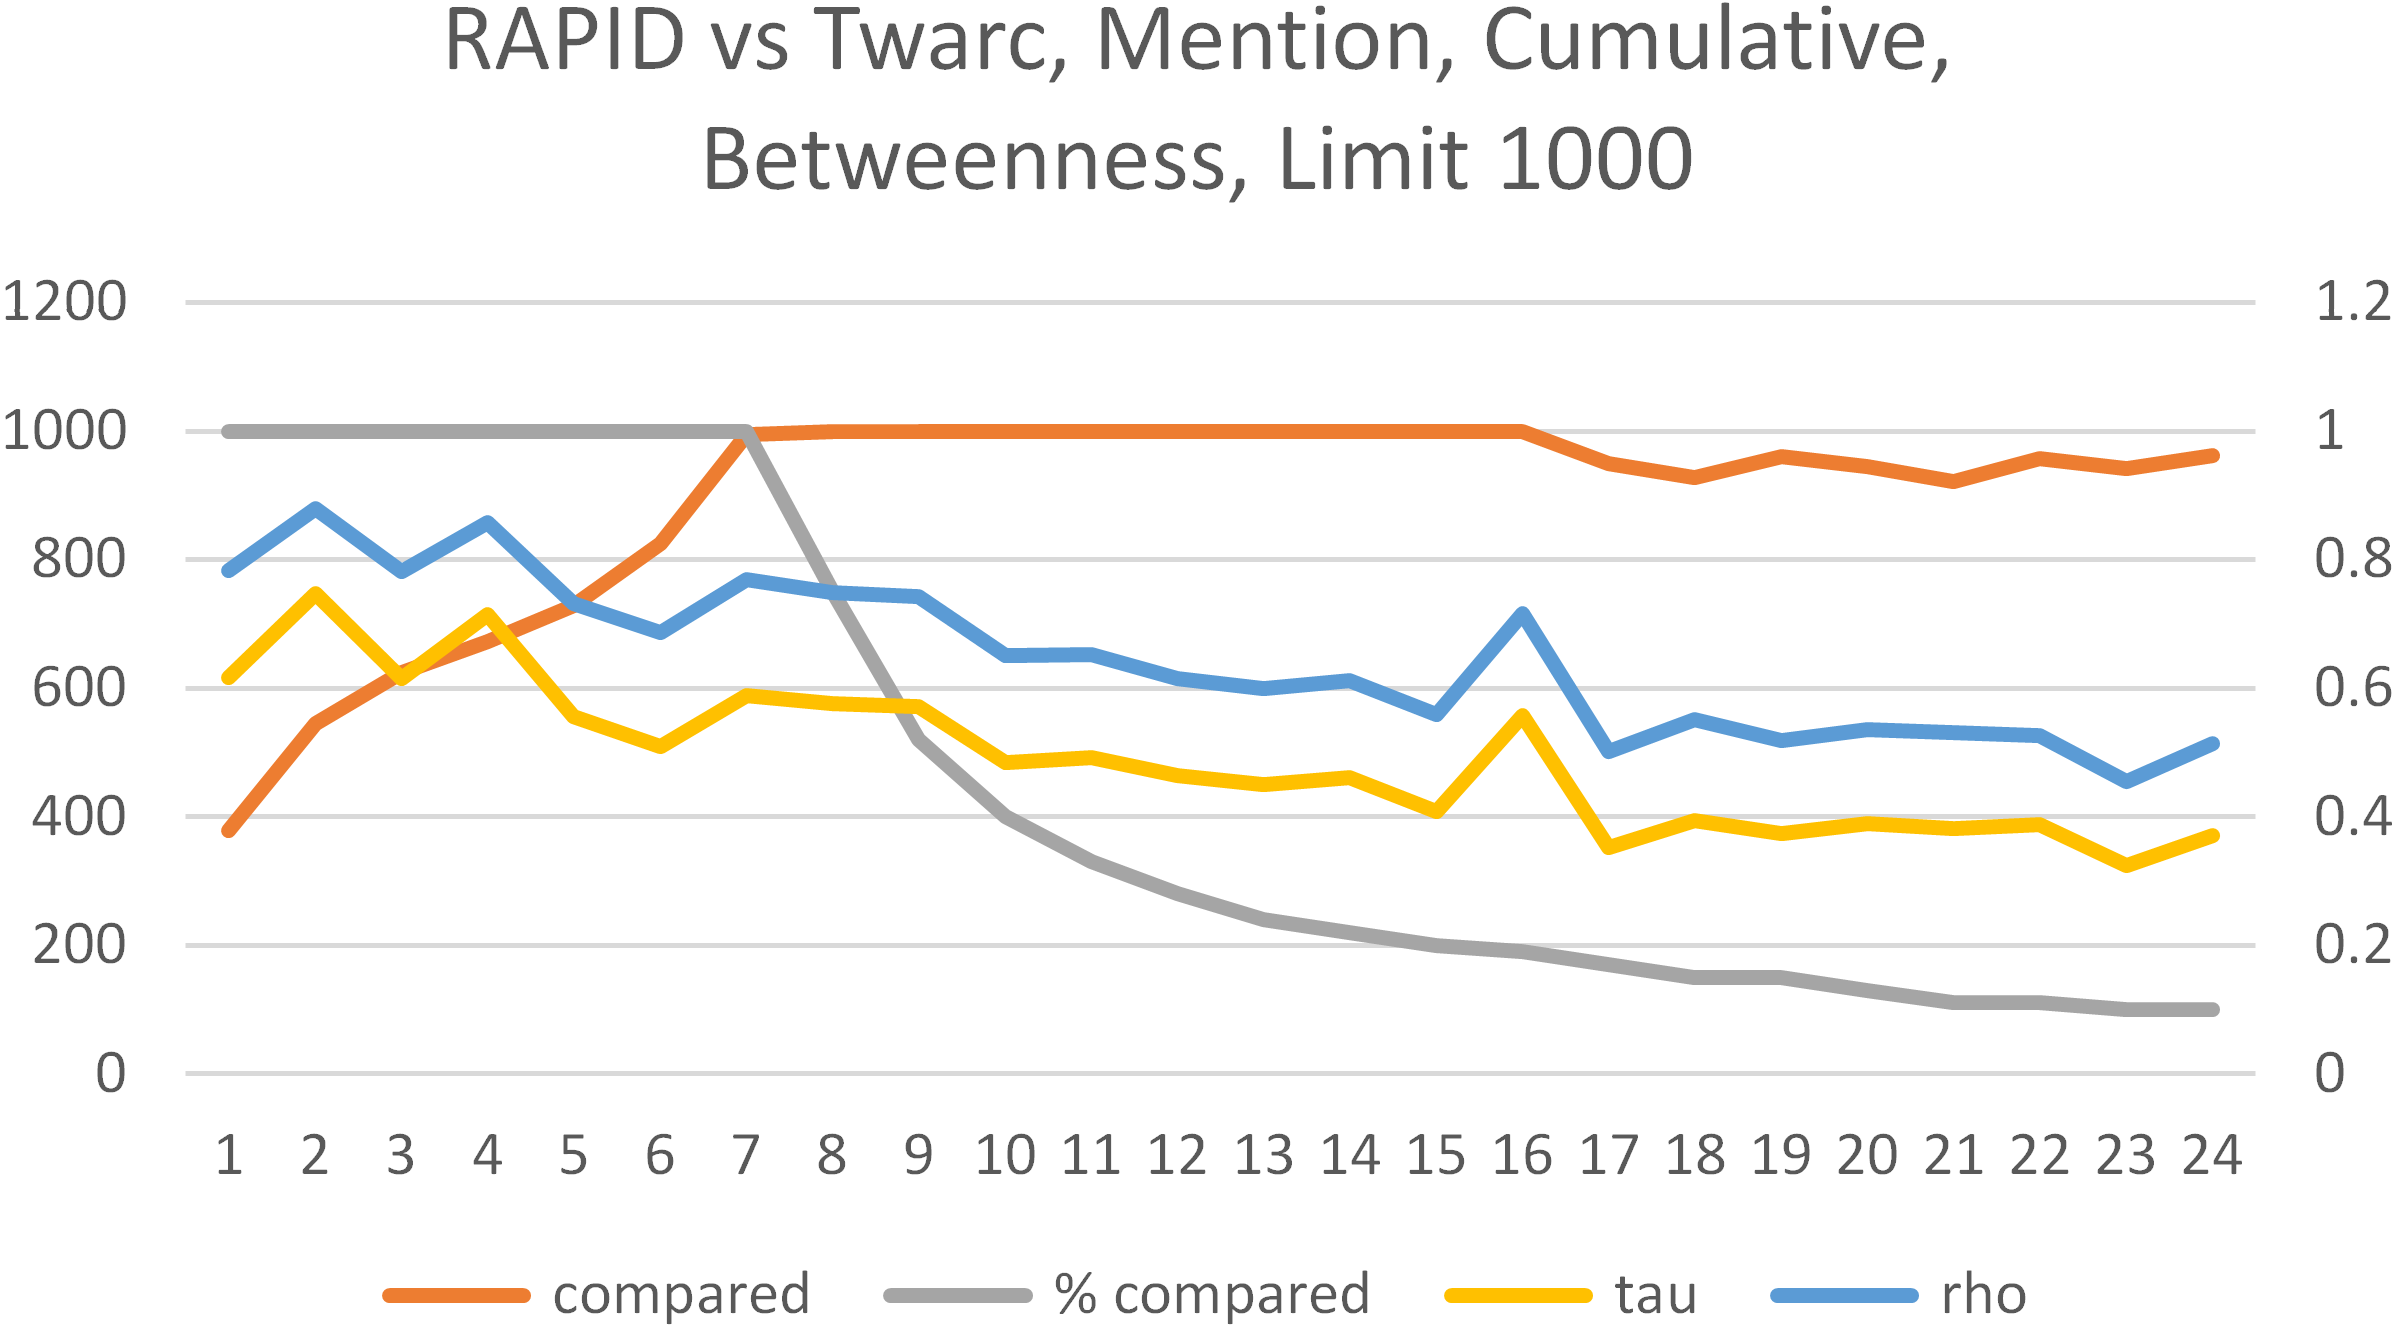}
        \caption{\tiny Mention/Betweenness.}
        \label{fig:elec_long_comparison_cumulative_men_bet}
    \end{subfigure}
    \hfill
    \begin{subfigure}[b]{0.3\textwidth}
        \centering
        \includegraphics[scale=0.11]{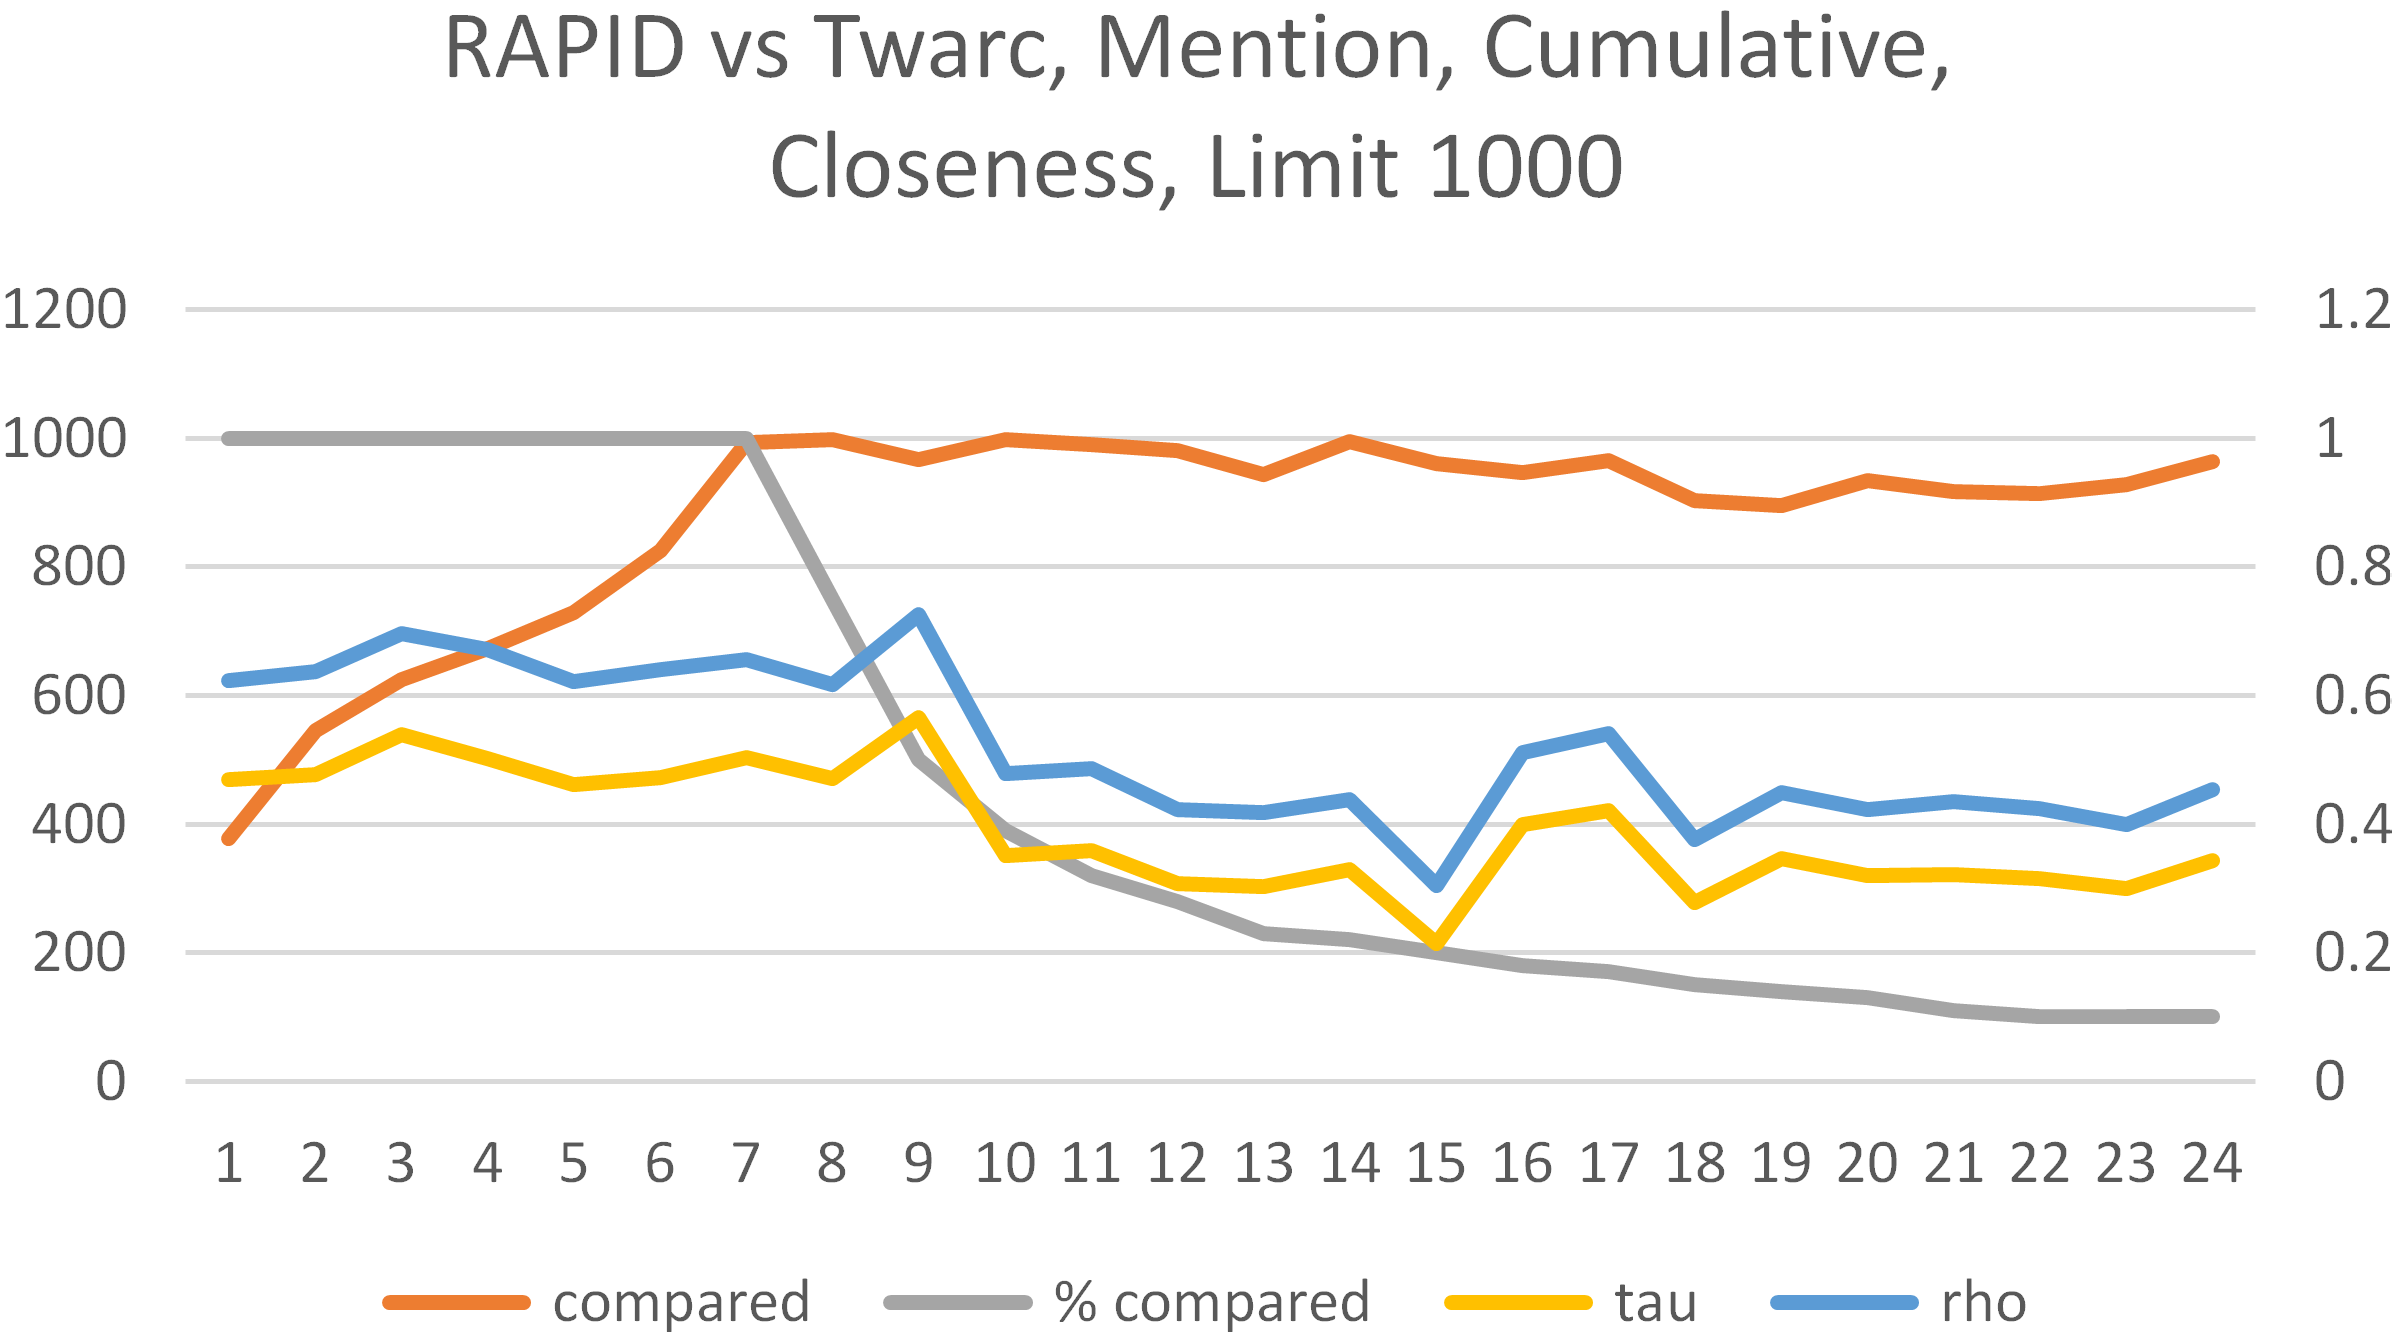}
        \caption{\tiny Mention/Closeness.}
        \label{fig:elec_long_comparison_cumulative_men_clo}
    \end{subfigure}
    
    \bigskip
    \begin{subfigure}[b]{0.3\textwidth}
        \centering
        \includegraphics[scale=0.11]{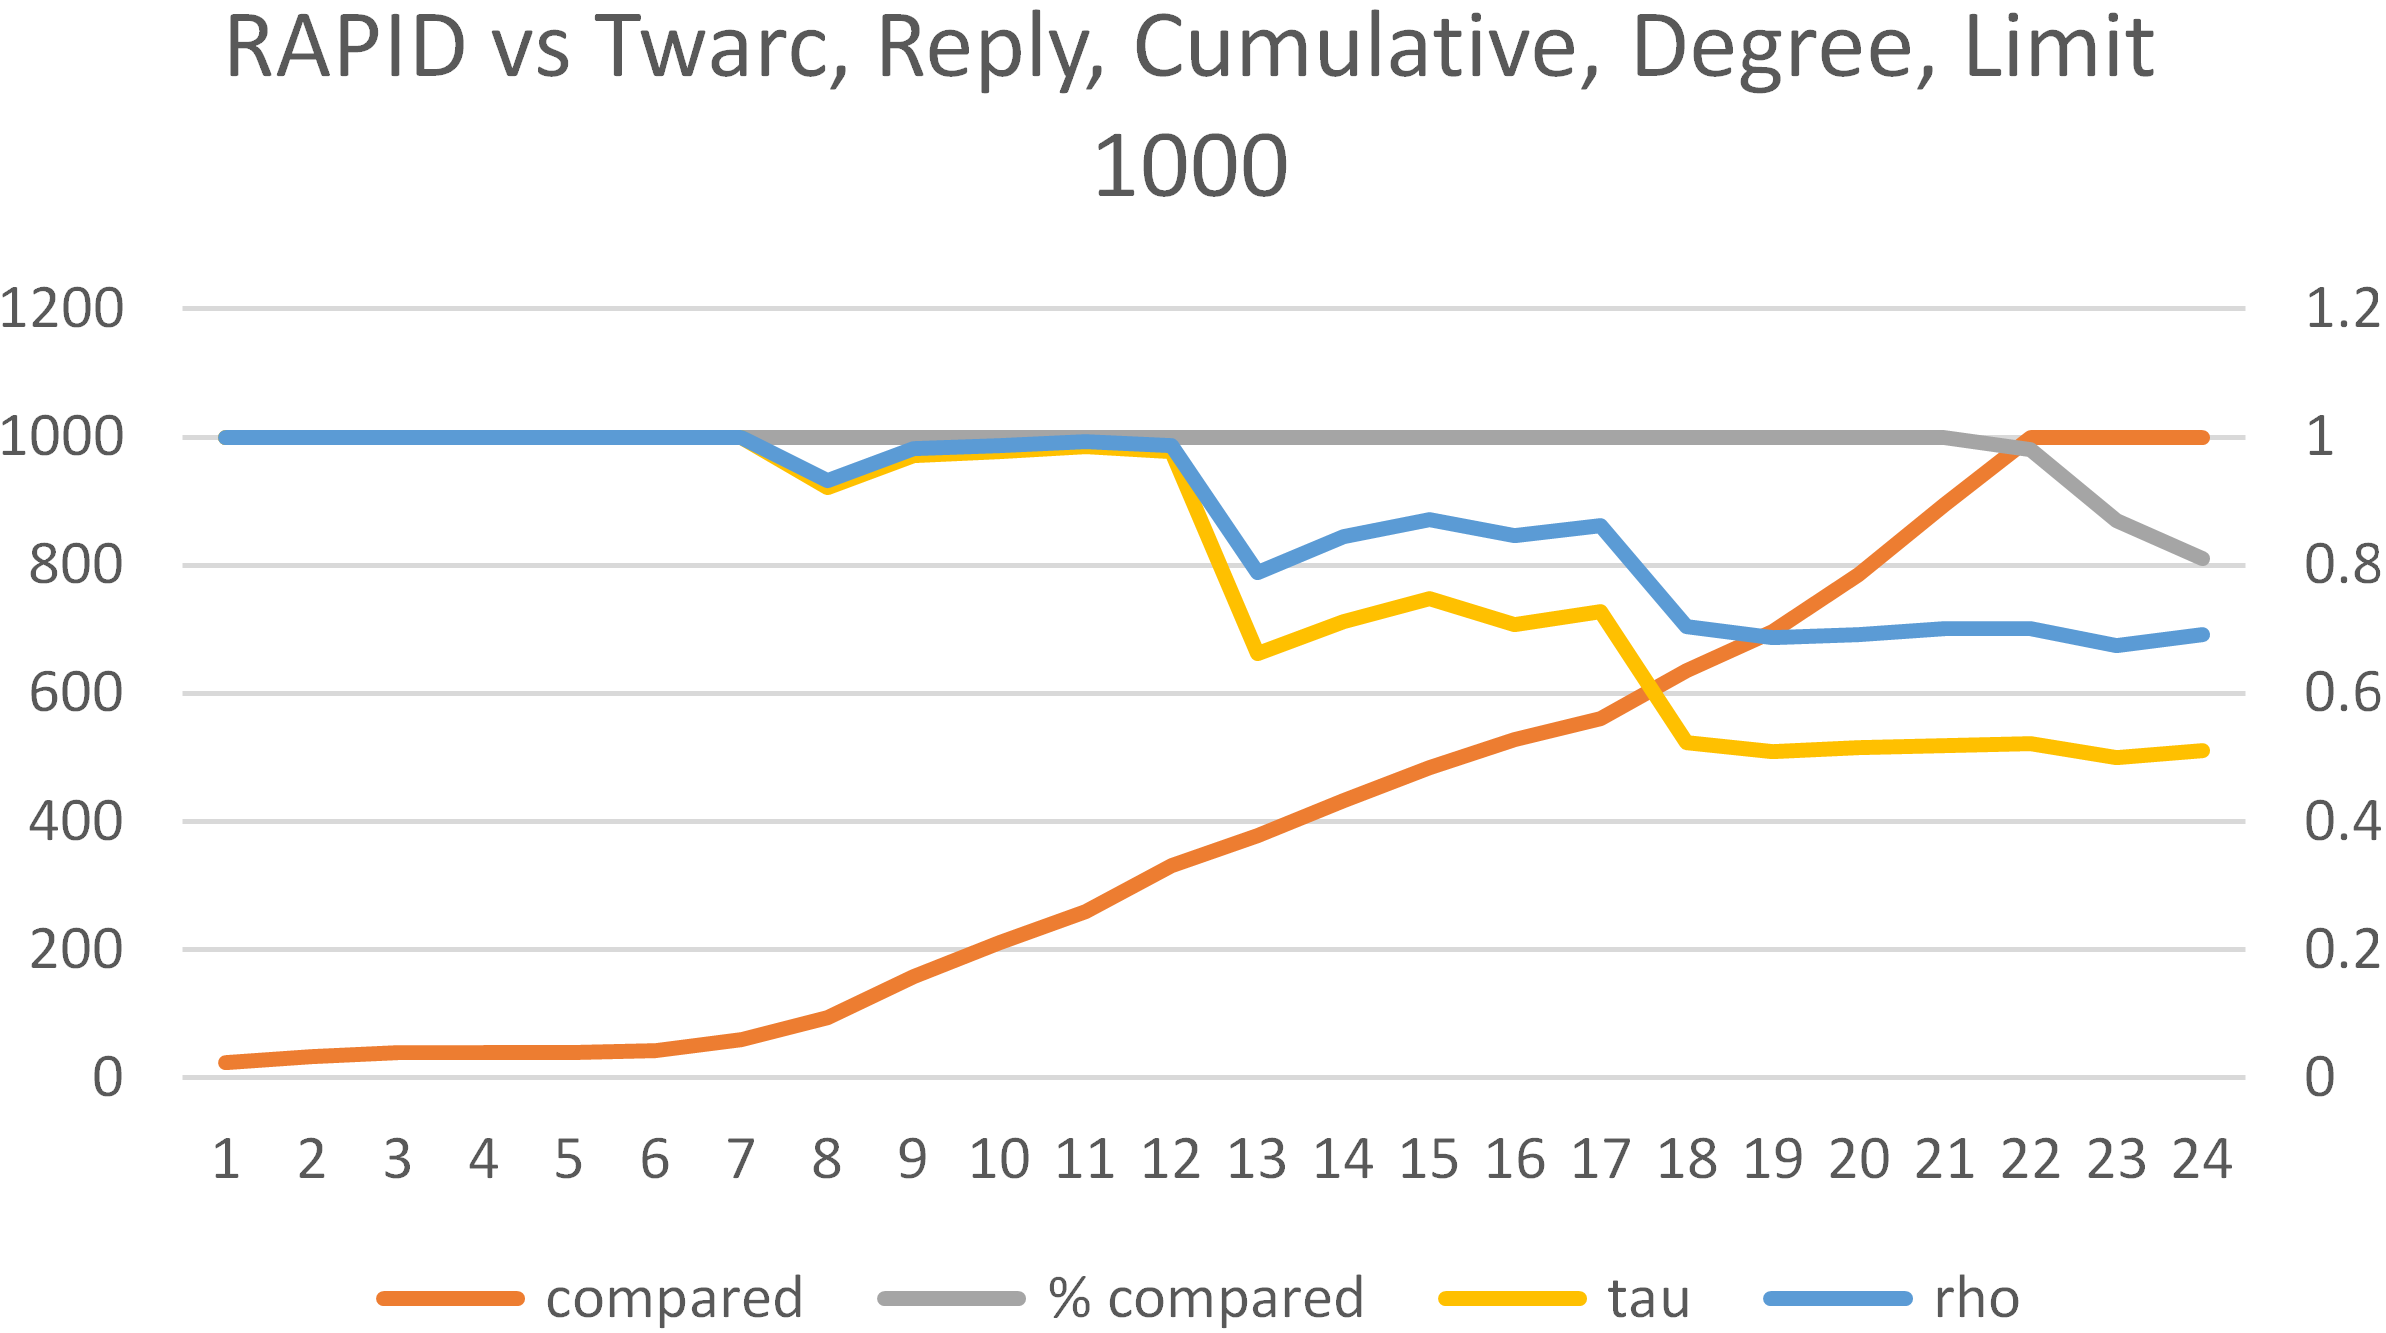}
        \caption{\tiny Reply/Degree.}
        \label{fig:elec_long_comparison_cumulative_rep_deg}
    \end{subfigure}
    \hfill
    \begin{subfigure}[b]{0.3\textwidth}
        \centering
        \includegraphics[scale=0.11]{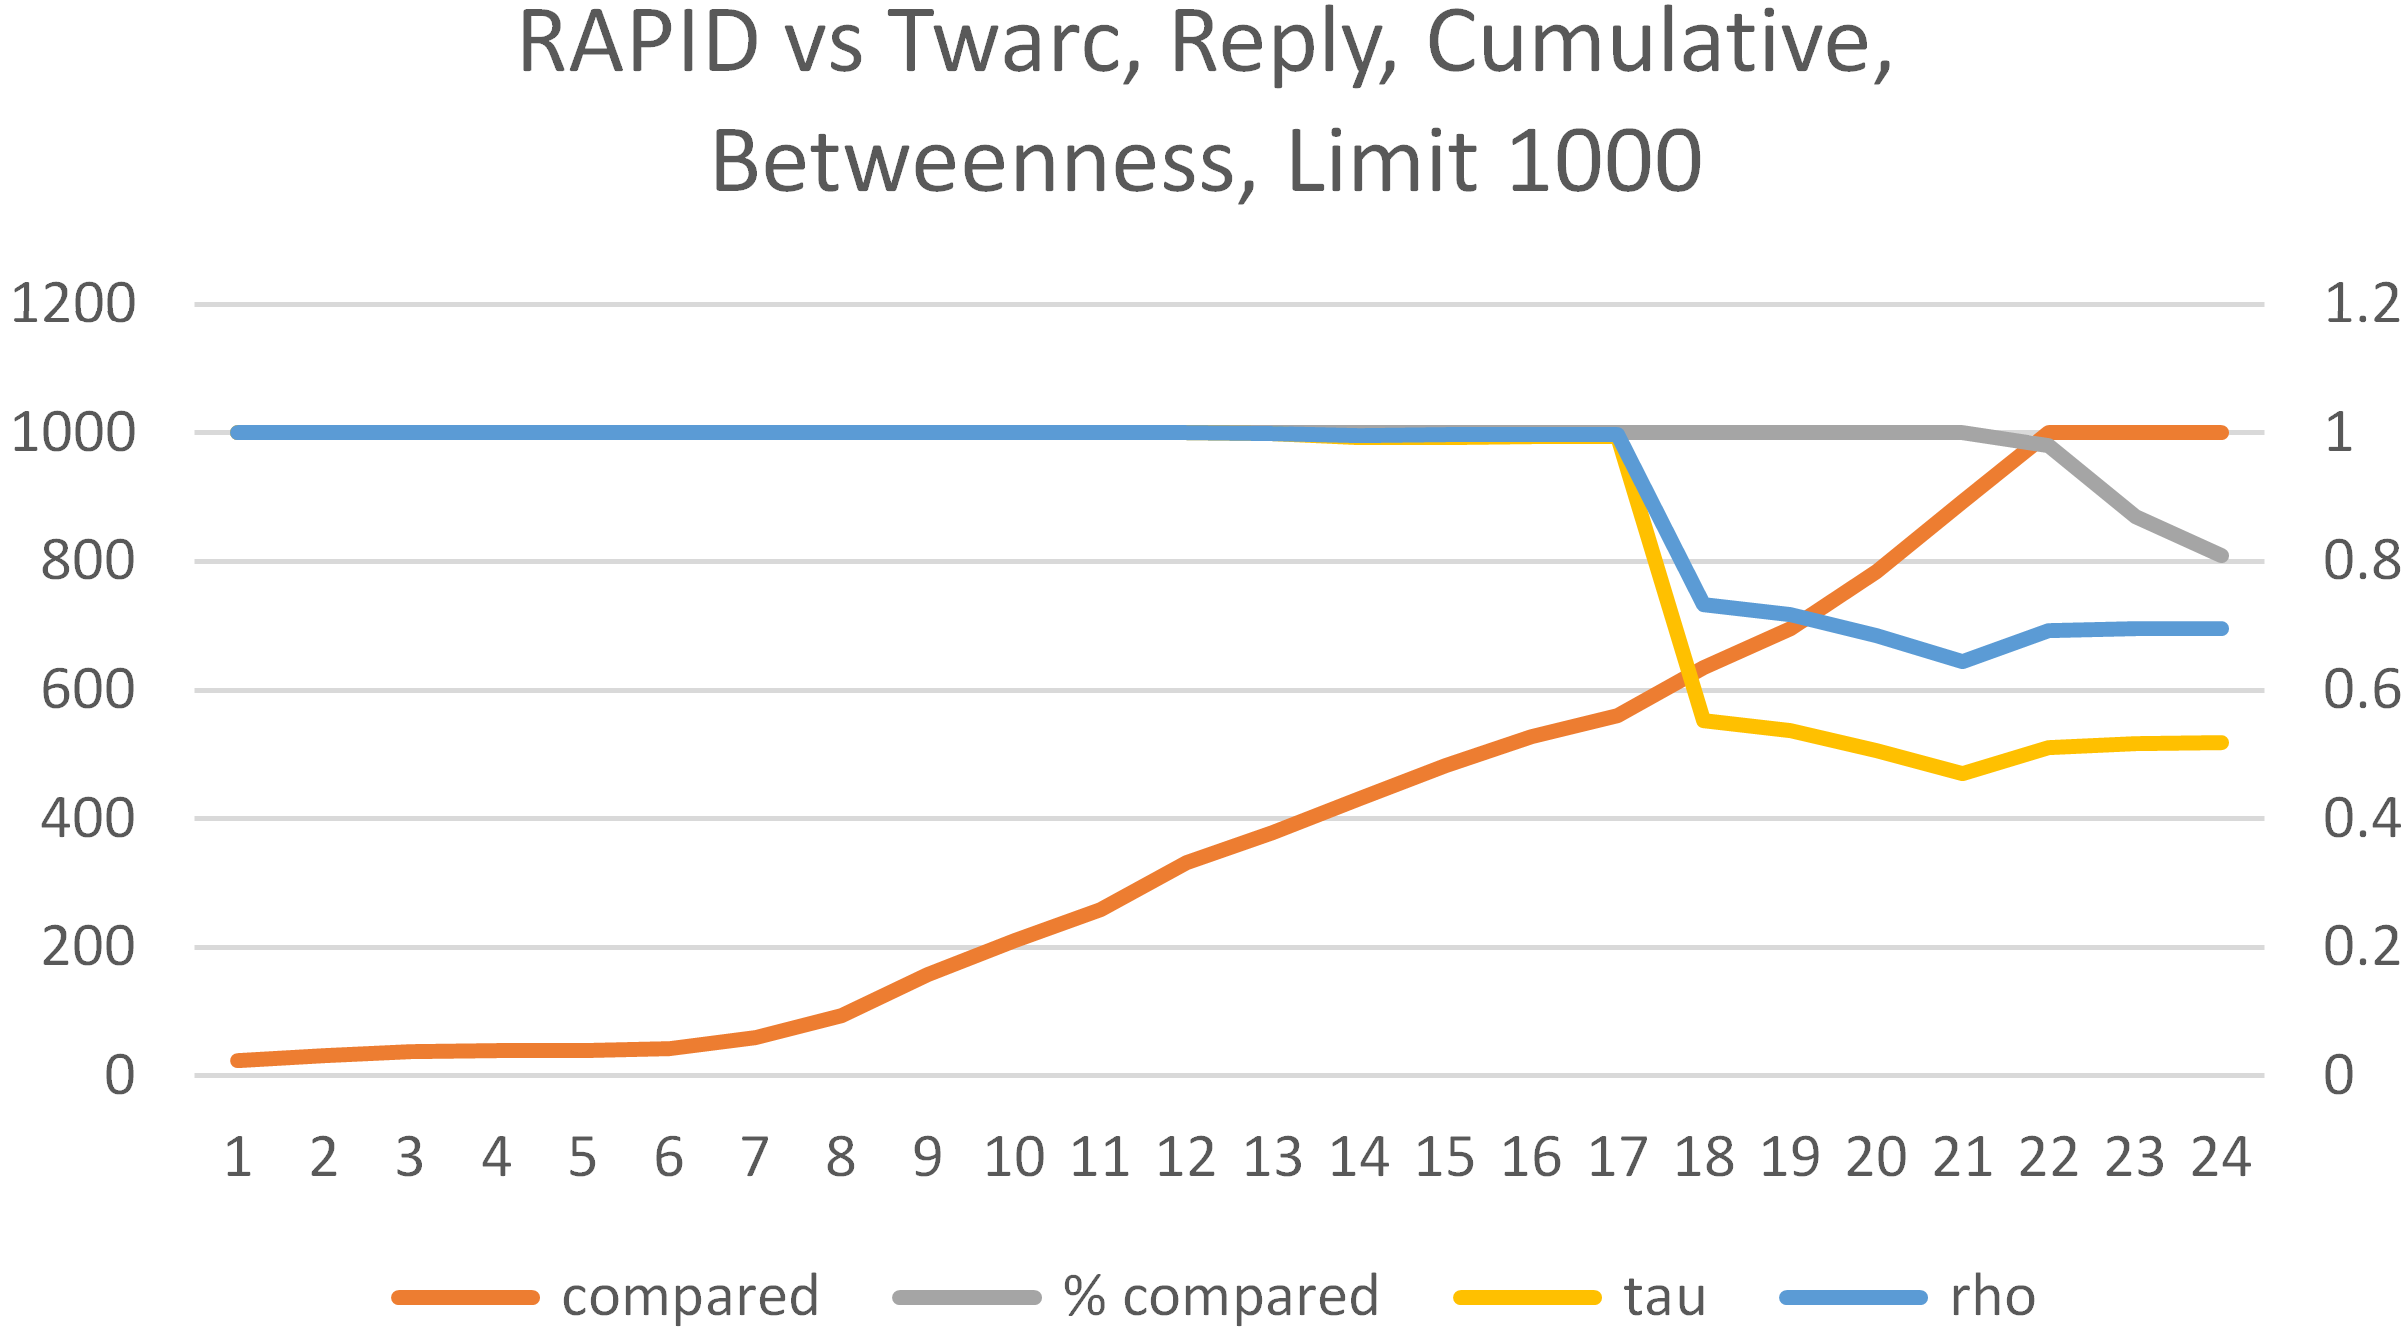}
        \caption{\tiny Reply/Betweenness.}
        \label{fig:elec_long_comparison_cumulative_rep_bet}
    \end{subfigure}
    \hfill
    \begin{subfigure}[b]{0.3\textwidth}
        \centering
        \includegraphics[scale=0.11]{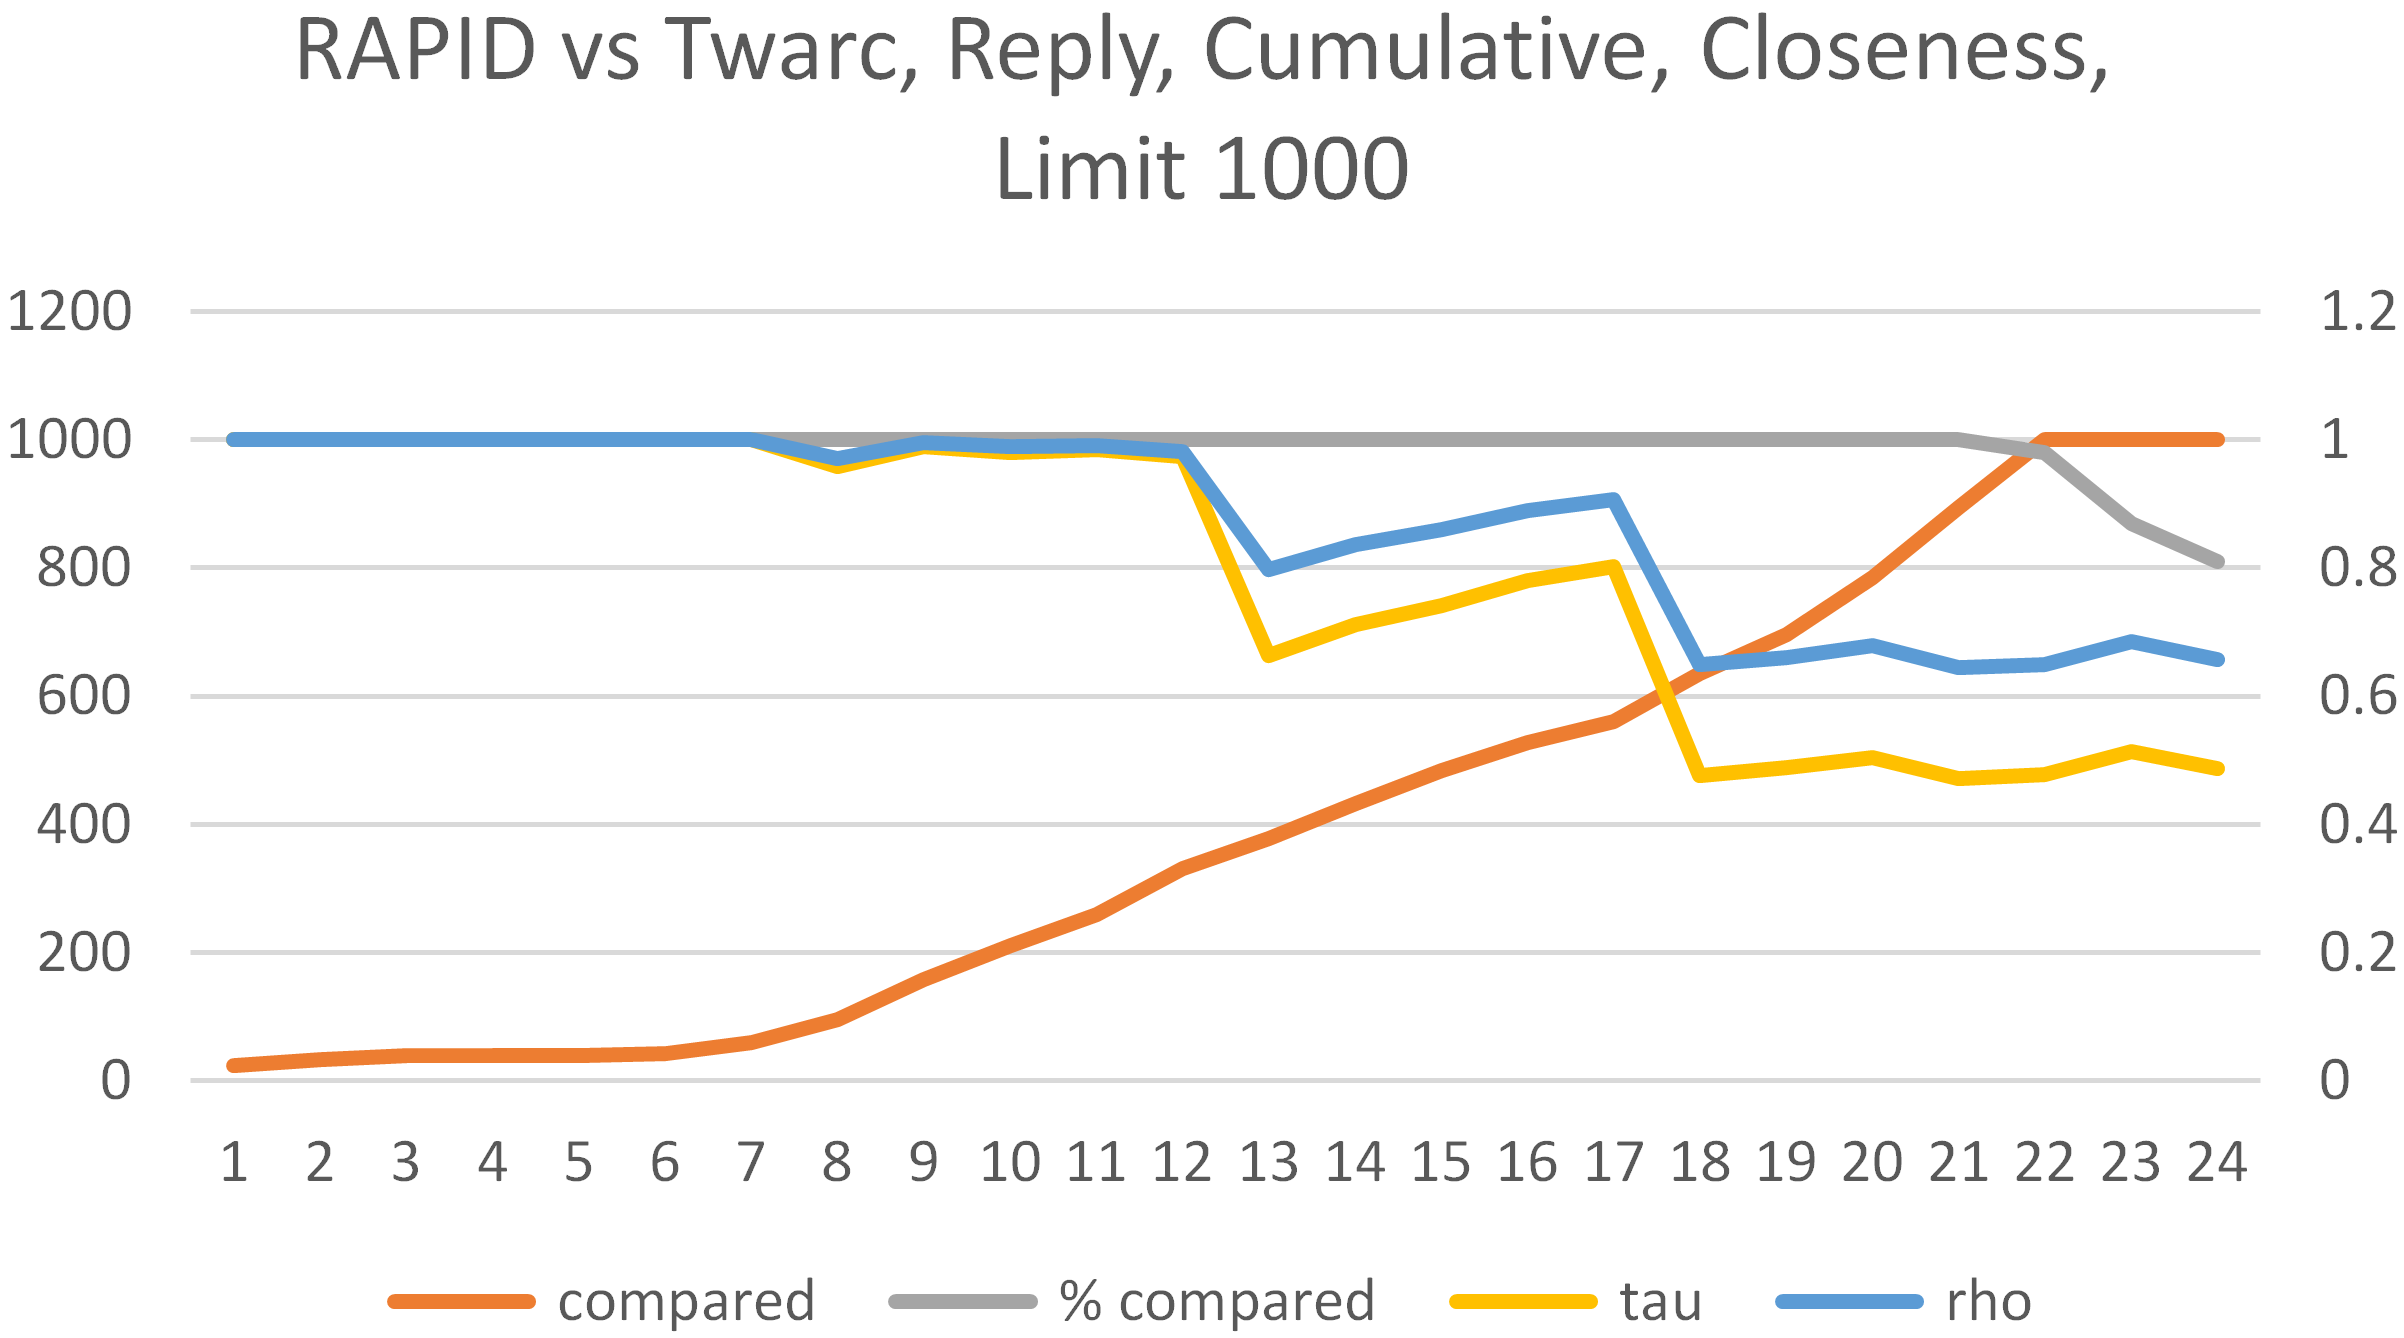}
        \caption{\tiny Reply/Closeness.}
        \label{fig:elec_long_comparison_cumulative_rep_clo}
    \end{subfigure}

    \caption{Cumulative longitudinal centrality ranking comparisons from the RAPID and Twarc datasets of the ``Election Day'' collections using Kendall Tau scores and Spearman's Coefficients.}
    \label{fig:elec_long_comparison_cumulative}
\end{figure}

\subsection{Case Study 3: Election Day}

A final collection for a case study was conducted but has been provided in the appendix due to space constraints and that fact that it did not show the considerable variation in collection tool performance observed in the previous case studies. The collection was conducted over an election day (24 hour period) in early 2019, using RAPID, Twarc and Tweepy, each configured with the same relevant filter terms. RAPID and Twarc collected slightly below 40k tweets each while Tweepy collected aroudn 36k tweets, but suffered from network outages on two occasions for approximately $60$--$90$ minutes each time (see Figure \ref{fig:nswelec_tweet_counts}). In the resulting datasets, 285 tweets were unique to RAPID, three to Twarc, and 19 were shared by Twarc and Tweepy but not RAPID. \marginpar{DCW has a venn diagram of this but it's not pretty}The vast majority of the Tweepy dataset, 36153 tweets, appeared in all three datasets, while Tweepy missed the 3118 further tweets that appeared in both Twarc and RAPID datasets. As these collections were so similar, we will not present their analyses here, but refer the reader to the \st{appendix} next subsection.

\begin{description}
    \item[Tweepy] Tweepy\footnote{\url{https://github.com/tweepy/tweepy}} is another Python library for communicating with the Twitter API, which also provides data in the JSON format.
\end{description}

\begin{figure}[ht!]
    \centering
    \includegraphics[scale=0.5]{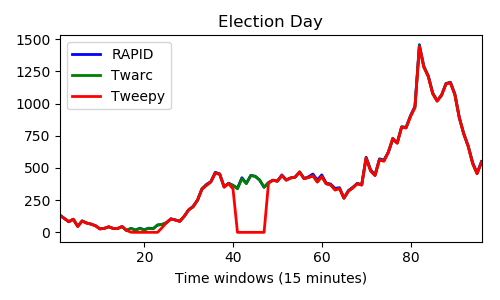}
    \caption{Tweet counts per 15 minutes in each of the datasets for the ``Election Day'' collection. The datasets track closely apart from two distinct interruptions in the Tweepy dataset.}
    \label{fig:nswelec_tweet_counts}
\end{figure}

%\noindent \emph{Election Day}: \\ A further collection tool, Tweepy, was introduced in the third and final collection, covering a period of significant online discussion over the twenty-four hour period of an election day in early 2019. Tweepy also provides a thin veneer between the user and Twitter's APIs, and the initial intent was to determine if Tweepy and Twarc provided near identical collections, however this could not be done due to network-related interruptions. Instead, it provides us with the ability to consider the effect of interruptions to collections.

% \begin{enumerate}
%     \item What effects on analyses are introduced when a collection is interrupted?
% \end{enumerate}

\subsubsection*{On the effects of interruptions}

\textbf{INTERRUPTIONS IN TWEEPY DURING ELECTION DAY}

\textit{Look at comparisons between Twarc and Tweepy to highlight how interruptions can affect your results.}

The above analyses highlight the differences between simultaneous collections conducted with different tools, but they are all assumed to be successful. As with any activity that inherently relies on networks, it is not unforeseeable that various connection issues may occur, and one element of social media data collection is to be able to identify and account for such interruptions. The comparisons for the ``Election Day'' collection have primarily focussed on the RAPID and Twarc collections, despite that the fact that Table \ref{tab:twitter_collections} makes it clear that Tweepy was used at the same time. Unfortunately the Tweepy collection activity suffered two interruptions, one of which appeared to last longer than an hour during the 24 hour collection period (Figure \ref{fig:nswelec_tweet_counts}).

% \begin{figure}[ht!]
%     \centering
%     \includegraphics[scale=0.5]{images/nswelec-rapid-k_twarc_tweepy-tweet_counts-15m.png}
%     \caption{Tweet counts per 15 minutes in each of the datasets for the ``Election Day'' collection. The datasets track closely apart from two distinct interruptions in the Tweepy dataset.}
%     \label{fig:nswelec_tweet_counts}
% \end{figure}

Here we explore how much of a difference such an interruption causes to the networks derived from the affected dataset.

\textbf{Centrality measures}

When contrasted with the comparisons the RAPID and Twarc dataset-derived centrality rankings (Figure \ref{fig:elec_centrality_ranking_comparisons_tau_rho}), the comparison of the Twarc and Tweepy dataset-derived centrality rankings shown in Figure \ref{fig:nswelec_interrupted_centrality_comparison} indicate a much greater discrepancy, as do the scatterplots of the rankings themselves, both raw (Figure \ref{fig:elec_interrupted_centrality_ranking_comparisons}) and with the rank score variation (Figure \ref{fig:elec_interrupted_centrality_ranking_comparisons2}).

\begin{figure}[ht!]
    \centering
    \includegraphics[scale=0.35]{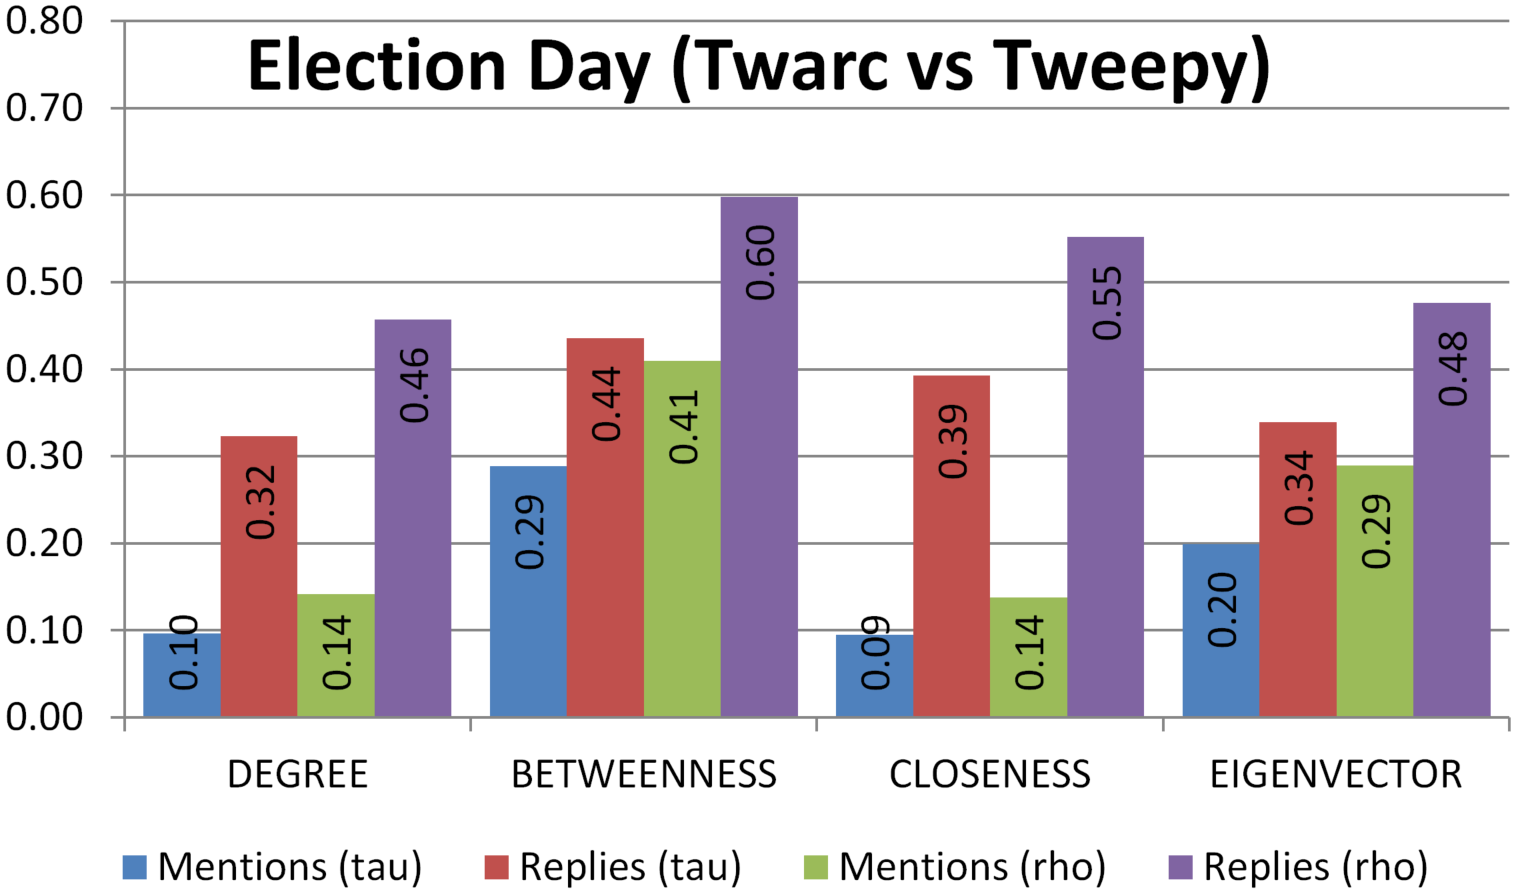}
    \caption{Centrality ranking comparisons for from the ``Election Day'' collection Twarc and Tweepy datasets. \emph{Cf.} the comparisons between the RAPID and Twarc datasets shown in Figure \ref{fig:elec_centrality_ranking_comparisons_tau_rho}.}
    \label{fig:nswelec_interrupted_centrality_comparison}
\end{figure}

\begin{figure}[ht!]
    \centering
    \includegraphics[scale=0.35]{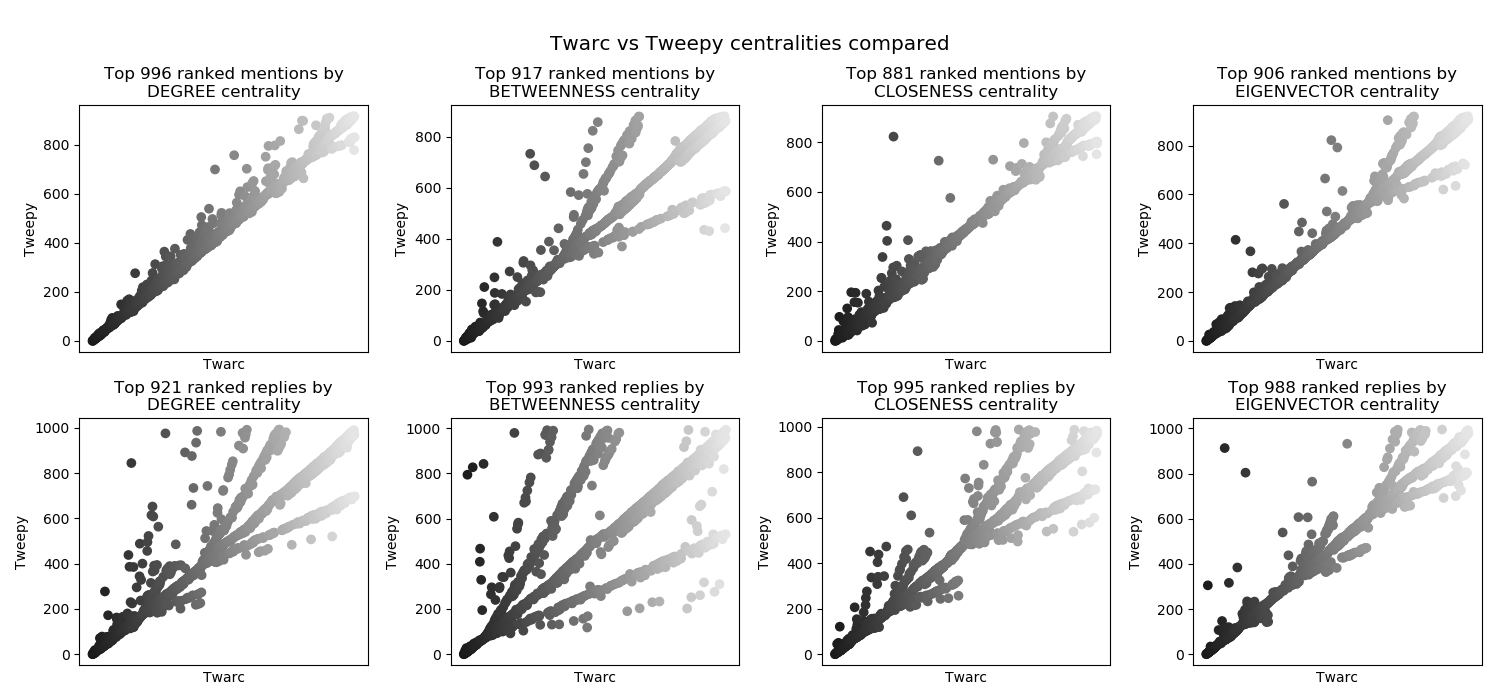}
    \caption{Centrality ranking scatterplot comparisons for from the ``Election Day'' collection Twarc and Tweepy datasets. \emph{Cf.} the comparisons between the RAPID and Twarc datasets shown in Figure \ref{fig:elec_centrality_ranking_comparisons}.}
    \label{fig:elec_interrupted_centrality_ranking_comparisons}
\end{figure}

\begin{figure}[ht!]
    \centering
    \includegraphics[scale=0.35]{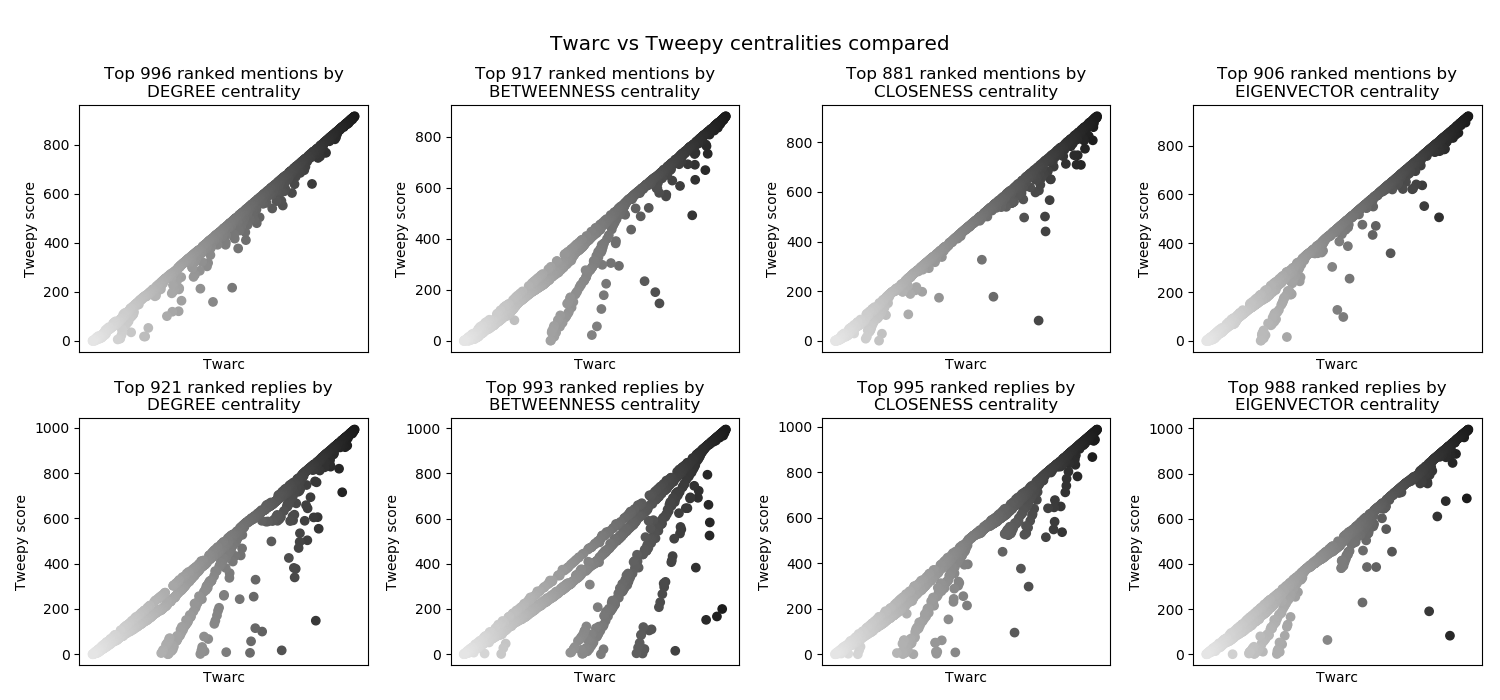}
    \caption{Centrality ranking comparison with the Nasim scores for from the ``Election Day'' collection Twarc and Tweepy datasets. \emph{Cf.} the comparisons between the RAPID and Twarc datasets shown in Figure \ref{fig:elec_centrality_ranking_comparisons2}.}
    \label{fig:elec_interrupted_centrality_ranking_comparisons2}
\end{figure}

\textbf{Longitudinal comparisons}

HOLD THIS BIT - CAN'T SEEM TO RUN THIS ON MY WINDOWS BOX, NEED scipy 1.2.2 WHICH HASN'T GOT TO ANACONDA YET - FOR SOME REASON THIS RUNS FINE ON MY MACBOOK THOUGH. HAVE TO TRANSFER FILES OVER...

To this point, the provided visualisations do not highlight the fact that there was a second interruption during collection. This is exposed to a greater when considering the rankings hour by hour, and it becomees clear that the lull, around the \nth{5} to \nth{6} hour, appears more likely to be a connection issue than simply a lack of activity. The reply and mention network comparisons also indicate a significant divergence in the membership of the networks as both Kendall $\tau$ and Spearman's coefficient values drop well below zero. (XXX IS THIS AN ERROR?!!!)

Longitudinal charts

\textbf{Community comparisons}

\begin{table}[ht]
    \centering\scriptsize
    \begin{tabular}{llrrc}
        \toprule
        Collection     & Interaction & Nodes & Edges &  ARI  \\
        \midrule
        Election Day   & RETWEET     &  8193 & 22286 & 0.396 \\
        (Twarc/Tweepy) & MENTION     &  9600 & 35235 & 0.602 \\
                       & REPLY       &  1147 &  1094 & 0.597 \\
        \bottomrule
    \end{tabular}
    \caption{Comparison of the communities found in the networks built from the Twarc and Tweepy Election Day datasets. The node count is the number of nodes in common between the networks, the edge count is drawn from the RAPID dataset in each case, to give an indication of density, and the ``ARI'' value is the Adjusted Rand index.}
    \label{tab:interrupted_community_comparison}
\end{table}

\newpage
